# Supplementary material for: A Bayesian joint model for mediation analysis with matrix-valued mediators
Source: arXiv:2310.00803 ancillary file (2024-09-24)
Supplement: Supplementary file 1 [file supplementary.pdf]

# Supplementary Materials for "A Bayesian Joint Model for Mediation Analysis with Matrix-Valued Mediators"

by

Zijin Liu, Zhihui (Amy) Liu, Ali Hosni, John Kim, Bei Jiang, and Olli Saarela

## Web Appendix A Likelihood

The full likelihood of our proposed joint model (1-3) in the main text is:

$$\begin{aligned} L(\Theta) &= \prod_{i=1}^{n} f(Y_i, \boldsymbol{X}_i, \boldsymbol{T}_i \mid E_i, \boldsymbol{Z}_i, \Theta) \\ &= \prod_{i=1}^{n} f(Y_i \mid \boldsymbol{T}_i, E_i, \boldsymbol{Z}_i, \Theta) f(\boldsymbol{X}_i \mid \boldsymbol{T}_i, \Theta) f(\boldsymbol{T}_i \mid E_i, \boldsymbol{Z}_i, \Theta) \\ &= \prod_{i=1}^{n} \Bigg[ p_i^{\mathcal{I}(Y_i=1)} (1-p_i)^{\mathcal{I}(Y_i=0)} \left(\frac{\phi}{2\pi}\right)^{pq/2} \exp\left(-\frac{\phi}{2} \left\| \boldsymbol{X}_i - \boldsymbol{\mu} - \boldsymbol{A}\boldsymbol{T}_i\boldsymbol{B}^\top \right\|_F^2\right) \\ &\quad \times \left(\frac{1}{2\pi}\right)^{p_0q_0/2} \exp\left(-\frac{1}{2}\left\| \mathrm{vec}(\boldsymbol{T}_i) - \boldsymbol{\beta}_{ET}E_i - \boldsymbol{\Omega}_{ZT}\boldsymbol{Z}_i \right\|^2\right)\Bigg] \end{aligned} \tag{A.1}$$

where $\|\cdot\|^2$ and $\|\cdot\|_F^2$ are Euclidean norm and Frobenius norm, respectively, and $p_i = \Phi(\alpha_Y + \beta_{EY}E_i + \boldsymbol{\beta}_{TY}^\top \mathrm{vec}(\boldsymbol{T}_i) + \boldsymbol{\beta}_{ZY}^\top \boldsymbol{Z}_i)$.

## Web Appendix B Derivation of Causal Decomposition Effects

We further denote $\mathrm{vec}(\boldsymbol{T}_i) = (T_i^1, \cdots, T_i^{p_0q_0})^\top$, and then define $T_i^j = T_i^j(e)$ as the $j$th potential vectorized latent feature for subject $i$ set to treatment level $E_i = e$. Similarly, define $Y_i(e^*, T_i^1(e), \cdots, T_i^{p_0q_0}(e))$ as the potential outcome $Y_i$ if $E_i = e^*$ and $T_i^j = T_i^j(e)$, for all $j = 1, \cdots, p_0q_0$.

Following Lange et al. (2014)'s causal assumptions for multiple mediators, for any treatment level pair $\{e, e^*\}$ where $e \neq e^*$, and any $j, j' \in \{1, \cdots, p_0q_0\}$, as well as any level of latent features $(t^1, \cdots, t^{p_0q_0}) \in \mathbb{R}^{p_0q_0}$, we assume

$$\{Y_i(e, t^1, \cdots, t^{p_0q_0}), T_i^j(e)\} \perp E_i \mid \boldsymbol{Z}_i \tag{B.1}$$

$$Y_i(e, t^1, \cdots, t^{p_0q_0}) \perp T_i^j \mid (E_i = e, \boldsymbol{Z}_i) \tag{B.2}$$

$$Y_i(e^*, t^1, \cdots, t^{p_0q_0}) \perp T_i^j(e) \mid \boldsymbol{Z}_i \tag{B.3}$$

$$T_i^j(e) \perp T_i^{j'}(e^*) \mid \boldsymbol{Z}_i \tag{B.4}$$

Assumptions (B.1) and (B.2) imply "no unmeasured confounding" of the exposure-mediator, exposure-outcome, and mediator-outcome relationships. In the context of our application, the safety outcomes we consider are not expected to be affected by confounding by indication. That is, our outcome, unplanned treatment interruption, is unlikely to be related to determinants of the prescription dose (exposure) or the dose distributions to organs-at-risk (mediator). Assumptions (B.3-B.4) mirror Lange et al. (2014)'s extended sequential ignorability assumptions for identifying causal effects. In particular, the "cross-world" independence assumption (B.3) can be interpreted to mean the absence of "exposure-induced mediator-outcome confounding". For the same reasons as for (B.1) and (B.2), and because of the small temporal separation between the exposure and the mediator, we do not expect violations of this assumption in the context of our application. The causal assumption (B.4) enables decomposition of the mediated effects into additive components operating through the different latent variables. This is satisfied through the modeling assumptions we make, as the latent mediator variables are taken to be independent in the MPCA model.

In addition to the causal assumptions (B.1)-(B.4), we define "consistency" and "positivity" assumptions similar to Lange et al. (2014). In our notation,

- **Consistency** states that if $E_i = e$ and $\text{vec}(\boldsymbol{T}_i) = \boldsymbol{t}$, the potential outcome $Y_i(e, \boldsymbol{t}) = Y_i$, that is, equal to the observed outcome, and similarly, if $E_i = e$, the potential mediator $\boldsymbol{T}_i(e) = \boldsymbol{T}_i$.

- **Positivity** assumes the following two inequalities hold: $0 < P(E_i = e \mid \boldsymbol{Z}_i = \boldsymbol{z}) < 1$ and $0 < P(T_i^j = t^j \mid E_i = e, \boldsymbol{Z}_i = \boldsymbol{z}) < 1$, $j = 1, \cdots, p_0q_0$, for all possible values of exposure $e$, latent features $t^j$, and covariates $\boldsymbol{z}$.

We decompose the total effect (TE) of changing treatment from $e^*$ to $e$ into (i) Natural direct effect (NDE), which captures how the treatment directly affects the outcome, and (ii) Natural indirect effect (NIE), which captures how the treatment affects the outcome through the latent features. NIE can be further partitioned into $j = 1, \cdots, p_0q_0$ pathways through $p_0q_0$ distinct latent features, denoted by $\text{NIE}_j$. Specifically, for $j = 1, \cdots, p_0q_0$,

$$\begin{aligned}
\text{NDE}(e, e^*) &= E[Y_i(e^*, T_i^1(e), \cdots, T_i^{p_0q_0}(e))] - E[Y_i(e, T_i^1(e), \cdots, T_i^{p_0q_0}(e))] \\
\text{NIE}_j(e, e^*) &= E[Y_i(e^*, T_i^1(e^*), \ldots, T_i^{j-1}(e^*), T_i^j(e^*), T_i^{j+1}(e), \ldots, T_i^{p_0q_0}(e)] \\
&\quad - E[Y_i(e^*, T_i^1(e^*), \ldots, T_i^{j-1}(e^*), T_i^j(e), T_i^{j+1}(e), \ldots, T_i^{p_0q_0}(e)] \\
\text{NIE}(e, e^*) &= E[Y_i(e^*, T_i^1(e^*), \cdots, T_i^{p_0q_0}(e^*))] - E[Y_i(e^*, T_i^1(e), \cdots, T_i^{p_0q_0}(e))] \\
&= \text{NIE}_1 + \cdots + \text{NIE}_{p_0q_0} \\
\text{TE} &= \text{NDE} + \text{NIE} = \text{NDE} + \text{NIE}_1 + \cdots + \text{NIE}_{p_0q_0}.
\end{aligned}$$

To compute these, we consider a general case $E[Y_i(e^0, T_i^1(e^1), \cdots, T_i^{p_0q_0}(e^{p_0q_0}))]$, where $e^0, e^1, \cdots, e^{p_0q_0} \in \{e, e^*\}$, and by g-computation, under Assumptions (B.1-B.4) we can show

that

$$E[Y_i(e^0, T_i^1(e^1), \cdots, T_i^{p_0q_0}(e^{p_0q_0}))]$$
$$= E_{\boldsymbol{Z}_i}\left\{\int_{\boldsymbol{t}} \Phi(\alpha_Y + \beta_{EY}e^0 + \boldsymbol{\beta}_{TY}^\top \boldsymbol{t} + \boldsymbol{\beta}_{ZY}^\top \boldsymbol{Z}_i) f_{T_i^1|E_i=e^1,\boldsymbol{Z}_i}(t^1)\cdots f_{T_i^{p_0q_0}|E_i=e^{p_0q_0},\boldsymbol{Z}_i}(t^{p_0q_0})\mathrm{d}\boldsymbol{t}\right\} \tag{B.5}$$

where $f_{T_i^j|E_i=e^j,\boldsymbol{Z}_i}(t^j)$ is the density function of $T_i^j$ conditional on $E_i = e^j$ and $\boldsymbol{Z}_i$, for $j = 1, \cdots, p_0q_0$, and $\boldsymbol{t} = (t^1, \cdots, t^{p_0q_0})^\top$. Based on submodel (2), we have $T_i^j \mid (E_i = e^j, \boldsymbol{Z}_i) \sim N(\beta_{ET,j}e^j + \sum_{k=1}^K \Omega_{jk}Z_{ik}, 1)$. Since these latent features are assumed to be mutually independent conditional on exposure and covariates, we can show that the joint distribution of $T_i^j \mid (E_i = e^1, \boldsymbol{Z}_i), \cdots, T_i^{p_0q_0} \mid (E_i = e^{p_0q_0}, \boldsymbol{Z}_i)$ is $N(\boldsymbol{\beta}_{ET} \circ \boldsymbol{e} + \boldsymbol{\Omega}_{ZT}\boldsymbol{Z}_i, \boldsymbol{I}_{p_0q_0})$, where $\boldsymbol{e} = (e^1, \cdots, e^{p_0q_0})^\top$ and $\circ$ is the element-wise (Hadamard) product. The derivation of Equation (B.5) is provided in the next paragraph. The integral inside the expectation in (B.5) can be approximated by Monte Carlo integration. For $s = 1, \cdots, S$, its Monte Carlo estimate is

$$\frac{1}{S}\sum_{s=1}^{S} \Phi\left(\alpha_Y + \beta_{EY}e^0 + \boldsymbol{\beta}_{TY}^\top \boldsymbol{t}^{(s)} + \boldsymbol{\beta}_{ZY}^\top \boldsymbol{Z}_i\right) \tag{B.6}$$

where $\boldsymbol{t}^{(s)}$ is the $s$th sample from $N(\boldsymbol{\beta}_{ET} \circ \boldsymbol{e} + \boldsymbol{\Omega}_{ZT}\boldsymbol{Z}_i, \boldsymbol{I}_{p_0q_0})$. Finally, the outer expectation in (B.5) can be computed by averaging over all the covariate values in the sample.

To derive identification results (B.5) for the decomposition effects, we first apply the law of total expectation to $E[Y_i(e^*, T_i^1(e), \cdots, T_i^{p_0q_0}(e))]$ twice over the covariates $\boldsymbol{Z}_i$ and latent features $T_i^1(e^1), \cdots, T_i^{p_0q_0}(e^{p_0q_0})$ conditional on $\boldsymbol{Z}_i$, respectively, and then expand the middle expectation (with respect to latent features) using integration by the definition of expectation, to give

$$\begin{aligned}
&E[Y_i(e^0, T_i^1(e^1), \cdots, T_i^{p_0q_0}(e^{p_0q_0}))] \\
&= E_{\boldsymbol{Z}_i}\{E(Y_i(e^0, T_i^1(e^1), \cdots, T_i^{p_0q_0}(e^{p_0q_0})) \mid \boldsymbol{Z}_i)\} \\
&= E_{\boldsymbol{Z}_i}\{E_{T_i^1(e^1),\cdots,T_i^{p_0q_0}(e^{p_0q_0})|\boldsymbol{Z}_i}[ \\
&\qquad E(Y_i(e^0, T_i^1(e^1), \cdots, T_i^{p_0q_0}(e^{p_0q_0})) \mid T_i^1(e^1) = t^1, \cdots, T_i^{p_0q_0}(e^{p_0q_0}) = t^{p_0q_0}, \boldsymbol{Z}_i)]\} \\
&= E_{\boldsymbol{Z}_i}\left\{\int_{\boldsymbol{t}} E(Y_i(e^0, T_i^1(e^1), \cdots, T_i^{p_0q_0}(e^{p_0q_0})) \mid T_i^1(e^1) = t^1, \cdots, T_i^{p_0q_0}(e^{p_0q_0}) = t^{p_0q_0}, \boldsymbol{Z}_i)\right. \\
&\qquad \left. \times f_{T_i^1(e^1),\cdots,T_i^{p_0q_0}(e^{p_0q_0})|\boldsymbol{Z}_i}(\boldsymbol{t})\mathrm{d}\boldsymbol{t}\right\}.
\end{aligned} \tag{B.7}$$

The inner expectation in equation (B.7) is given by

$$E(Y_i(e^0, T_i^1(e^1), \cdots, T_i^{p_0q_0}(e^{p_0q_0})) \mid T_i^1(e^1) = t^1, \cdots, T_i^{p_0q_0}(e^{p_0q_0}) = t^{p_0q_0}, \boldsymbol{Z}_i) \tag{B.8a}$$
$$= E(Y_i(e^0, t^1, \cdots, t^{p_0q_0}) \mid T_i^1(e^1) = t^1, \cdots, T_i^{p_0q_0}(e^{p_0q_0}) = t^{p_0q_0}, \boldsymbol{Z}_i) \tag{B.8b}$$
$$= E(Y_i(e^0, t^1, \cdots, t^{p_0q_0}) \mid \boldsymbol{Z}_i) \tag{B.8c}$$
$$= E(Y_i(e^0, t^1, \cdots, t^{p_0q_0}) \mid E_i = e^0, T_i^1 = t^1, \cdots, T_i^{p_0q_0} = t^{p_0q_0}, \boldsymbol{Z}_i) \tag{B.8d}$$

$$= E(Y_i \mid E_i = e^0, T_i^1 = t^1, \cdots, T_i^{p_0q_0} = t^{p_0q_0}, \boldsymbol{Z}_i) \tag{B.8e}$$

$$= \Phi(\alpha_Y + \beta_{EY}e^0 + \boldsymbol{\beta}_{TY}^\top \boldsymbol{t} + \boldsymbol{\beta}_{ZY}^\top \boldsymbol{Z}_i), \tag{B.8f}$$

where the definition of conditional expectation is used from (B.8a) to (B.8b), the assumption (B.3) is used from (B.8b) to (B.8c), assumptions (B.1) and (B.2) are used from (B.8c) to (B.8d), and the consistency assumption is used from (B.8d) to (B.8e), followed by model (3) from (B.8e) to (B.8f).

The conditional joint density function in (B.7) is given by

$$\begin{aligned} f_{T_i^1(e^1),\cdots,T_i^{p_0q_0}(e^{p_0q_0})|\boldsymbol{Z}_i}(\boldsymbol{t}) &= f_{T_i^1(e^1)|\boldsymbol{Z}_i}(t^1)\cdots f_{T_i^{p_0q_0}(e^{p_0q_0})|\boldsymbol{Z}_i}(t^{p_0q_0}) && \text{(B.9a)} \\ &= f_{T_i^1(e^1)|E_i=e^1,\boldsymbol{Z}_i}(t^1)\cdots f_{T_i^{p_0q_0}(e^{p_0q_0})|E_i=e^{p_0q_0},\boldsymbol{Z}_i}(t^{p_0q_0}) && \text{(B.9b)} \\ &= f_{T_i^1|E_i=e^1,\boldsymbol{Z}_i}(t^1)\cdots f_{T_i^{p_0q_0}|E_i=e^{p_0q_0},\boldsymbol{Z}_i}(t^{p_0q_0}), && \text{(B.9c)} \end{aligned}$$

where Assumption (B.4) is used in (B.9a), Assumption (B.1) is used from (B.9a) to (B.9b), and the consistency assumption is used from (B.9b) to (B.9c). Letting $\dot{T}_i^j$ denote $T_i^j \mid E_i = e^j, \boldsymbol{Z}_i$, for $j = 1, \cdots, p_0q_0$, model (2) implies that (i) $\dot{T}_i^j \sim N(\beta_{ET,j}e^j + \sum_{k=1}^K \Omega_{jk}Z_{ik}, 1)$ and that (ii) $\dot{T}_i^j$ are mutually independent for any $j$. Subsequently, $(\dot{T}_i^1, \cdots, \dot{T}_i^{p_0q_0})^\top \sim N(\boldsymbol{\beta}_{ET} \circ \boldsymbol{e} + \boldsymbol{\Omega}_{ZT}\boldsymbol{Z}_i, \boldsymbol{I}_{p_0q_0})$, where $\boldsymbol{e} = (e^1, \cdots, e^{p_0q_0})^\top$, and $\circ$ is the element-wise (Hadamard) product. Thus, followed by (B.9c),

$$T_i^1(e^1), \cdots, T_i^{p_0q_0}(e^{p_0q_0}) \mid \boldsymbol{Z}_i \sim N(\boldsymbol{\beta}_{ET} \circ \boldsymbol{e} + \boldsymbol{\Omega}_{ZT}\boldsymbol{Z}_i, \boldsymbol{I}_{p_0q_0}). \tag{B.10}$$

Substituting equations (B.8f) and (B.10) into (B.7) completes the derivation of (B.5).

# Web Appendix C Gibbs sampling algorithm

Letting $\theta \mid \cdot$ denote the full conditional posterior distribution for the parameter $\theta$, updating $\boldsymbol{A} \mid \cdot$ and $\boldsymbol{B} \mid \cdot$ follows directly by the same procedure as in Jiang et al. (2020). Let $\boldsymbol{A}_{[,j]}$, $\boldsymbol{A}_{[,-j]}$, and $\boldsymbol{N}_{A_{[,-j]}}$ be the $j$th column of $\boldsymbol{A}$, $\boldsymbol{A}$ with its $j$th column removed, and an orthonormal basis for the null space of columns of $\boldsymbol{A}_{[,-j]}$, respectively. From Hoff (2007), $\boldsymbol{A}_{[,j]} \mid \boldsymbol{A}_{[,-j]} \overset{\text{d}}{=} \boldsymbol{N}_{A_{[,-j]}}\boldsymbol{a}_j$, where $\boldsymbol{a}_j$ follows a von Mises-Fisher distribution (denoted by vMF) with parameter $\boldsymbol{0}$. This provides a crucial tool to derive the full conditional posterior distribution of $\boldsymbol{A}_{[,j]}$, which is explicitly described in the Jiang et al. (2020)'s supplementary material 4.2. Similar notations can also be introduced for $\boldsymbol{B}$ (i.e. $\boldsymbol{B}_{[,k]}$, $\boldsymbol{B}_{[,-k]}$, and $\boldsymbol{N}_{B_{[,-k]}}$) with similar properties.

To implement Gibbs sampling for a probit model, we introduce a latent outcome variable $O_i$, such that $Y_i = \mathcal{I}(O_i > 0)$. Based on the joint model component (3), we can easily show that

$$\begin{aligned} \Pr(Y_i = 1 \mid E_i, \boldsymbol{T}_i, \boldsymbol{Z}_i) &= \Pr(O_i > 0 \mid E_i, \boldsymbol{T}_i, \boldsymbol{Z}_i) \\ &= \Phi(\alpha_Y + \beta_{EY}E_i + \boldsymbol{\beta}_{TY}^\top \text{vec}(\boldsymbol{T}_i) + \boldsymbol{\beta}_{ZY}^\top \boldsymbol{Z}_i), \end{aligned} \tag{C.1}$$

which indicates $O_i|E_i, \boldsymbol{T}_i, \boldsymbol{Z}_i \sim N(\alpha_Y + \beta_{EY}E_i + \boldsymbol{\beta}_{TY}^\top \text{vec}(\boldsymbol{T}_i) + \boldsymbol{\beta}_{ZY}^\top \boldsymbol{Z}_i, 1)$. We can then sample $O_i$ based on its the full conditional posterior distribution. For other model parameters,

conjugate priors are used and deriving their full conditional posterior distributions follows a standard procedure. In summary, our Gibbs sampling algorithm is:

- **Step 1:** Update $\boldsymbol{A}_{[,j]} \mid \cdot \overset{\mathrm{d}}{=} \boldsymbol{N}_{A_{[,-j]}} \widetilde{\boldsymbol{a}}_j$ for $j = 1, ..., p_0$. $\widetilde{\boldsymbol{a}}_j \sim \mathrm{vMF}(\phi \boldsymbol{N}_{A_{[,-j]}}^\top \sum_{i=1}^n \sum_{k=1}^{q_0} \boldsymbol{T}_{i[j,k]} \boldsymbol{X}_i^{-j} \boldsymbol{B}_{[,k]})$, where $\boldsymbol{X}_i^{-j} = \boldsymbol{X}_i - \boldsymbol{\mu} - \boldsymbol{A}_{[,-j]} \boldsymbol{T}_{i[-j,]} \boldsymbol{B}^\top$, $\boldsymbol{T}_{i[j,k]}$ represents the $(j,k)$th element of $\boldsymbol{T}_i$, and $\boldsymbol{T}_{i[-j,]}$ represents $\boldsymbol{T}_i$ with its $j$th row removed.

- **Step 2:** Update $\boldsymbol{B}_{[,k]} \mid \cdot \overset{\mathrm{d}}{=} \boldsymbol{N}_{B_{[,-k]}} \widetilde{\boldsymbol{b}}_k$ for $k = 1, ..., q_0$. $\widetilde{\boldsymbol{b}}_k \sim \mathrm{vMF}(\phi \boldsymbol{N}_{B_{[,-k]}}^\top \sum_{i=1}^n \sum_{j=1}^{p_0} \boldsymbol{T}_{i[j,k]} \widetilde{\boldsymbol{X}}_i^{-k} \boldsymbol{A}_{[,j]})$, where $\widetilde{\boldsymbol{X}}_i^{-k} = \boldsymbol{X}_i^\top - \boldsymbol{\mu}^\top - \boldsymbol{B}_{[,-k]} \boldsymbol{T}_{i[,-k]}^\top \boldsymbol{A}^\top$, and $\boldsymbol{T}_{i[,-k]}$ represents $\boldsymbol{T}_i$ with its $k$th column removed.

- **Step 3:** Update $\mathrm{vec}(\boldsymbol{T}_i) \mid \cdot \sim N(\boldsymbol{m}_i, \boldsymbol{C})$ for $i = 1, ..., n$, where $\boldsymbol{m}_i = \boldsymbol{C}[\phi(\boldsymbol{B} \otimes \boldsymbol{A})^\top (\mathrm{vec}(\boldsymbol{X}_i) - \mathrm{vec}(\boldsymbol{\mu})) + (\boldsymbol{\beta}_{ET} E_i + \boldsymbol{\Omega}_{ZT} \boldsymbol{Z}_i) + \boldsymbol{\beta}_{TY}(O_i - \alpha_Y - \beta_{EY} E_i - \boldsymbol{\beta}_{ZY}^\top \boldsymbol{Z}_i)]$ and $\boldsymbol{C} = [\boldsymbol{\beta}_{TY} \boldsymbol{\beta}_{TY}^\top + (1+\phi) \boldsymbol{I}_{p_0 q_0}]^{-1}$

- **Step 4:** Update $\phi \mid \cdot \sim \mathrm{Gamma}(a_0 + npq/2, b_0 + \sum_{i=1}^n \|\boldsymbol{X}_i - \boldsymbol{\mu} - \boldsymbol{A}\boldsymbol{T}_i\boldsymbol{B}^\top\|_F^2/2)$.

- **Step 5:** Update $\mathrm{vec}(\boldsymbol{\mu}) \mid \cdot \sim N\left(\sum_{i=1}^n \left[\mathrm{vec}(\boldsymbol{X}_i) - (\boldsymbol{B} \otimes \boldsymbol{A}) \mathrm{vec}(\boldsymbol{T}_i)\right]/n, (n\phi \boldsymbol{I}_{pq})^{-1}\right)$.

- **Step 6:** Update $\boldsymbol{\beta}_{ET} \mid \cdot \sim N\left(\boldsymbol{\Gamma}[\sum_{i=1}^n E_i(\mathrm{vec}(\boldsymbol{T}_i) - \boldsymbol{\Omega}_{ZT} \boldsymbol{Z}_i)], \boldsymbol{\Gamma}\right)$, where $\boldsymbol{\Gamma} = [(\gamma_0 \boldsymbol{I}_{p_0 q_0})^{-1} + \sum_{i=1}^n E_i^2 \boldsymbol{I}_{p_0 q_0}]^{-1}$.

- **Step 7:** Update $\boldsymbol{\Omega}_k \mid \cdot \sim N(\widetilde{\boldsymbol{\Gamma}}_k[\sum_{i=1}^n Z_{ik}(\mathrm{vec}(\boldsymbol{T}_i) - \boldsymbol{\beta}_{ET} E_i - \boldsymbol{\Omega}_{ZT[,-k]} \boldsymbol{Z}_{i[-k]})], \widetilde{\boldsymbol{\Gamma}}_k)$ for $k = 1, \cdots, K$, where $\widetilde{\boldsymbol{\Gamma}}_k = [(\gamma_0 \boldsymbol{I}_{p_0 q_0})^{-1} + \sum_{i=1}^n Z_{ik}^2 \boldsymbol{I}_{p_0 q_0}]^{-1}$, $\boldsymbol{\Omega}_{ZT[,-k]}$ is $\boldsymbol{\Omega}_{ZT}$ with its $k$th column $\boldsymbol{\Omega}_k$ removed, and $\boldsymbol{Z}_{i[-k]}$ is $\boldsymbol{Z}_i$ with its $k$th element $Z_{ik}$ removed.

- **Step 8:** Update $\boldsymbol{\beta}_Y = (\alpha_Y, \beta_{EY}, \boldsymbol{\beta}_{TY}^\top, \boldsymbol{\beta}_{ZY}^\top)^\top \mid \cdot \sim N(\boldsymbol{\Lambda} \sum_{i=1}^n \widetilde{\boldsymbol{Z}}_i O_i, \boldsymbol{\Lambda})$, where $\boldsymbol{\Lambda} = (\tau_0^{-1} \boldsymbol{I}_{p_0 q_0 + K + 2} + \sum_{i=1}^n \widetilde{\boldsymbol{Z}}_i \widetilde{\boldsymbol{Z}}_i^\top)^{-1}$, and $\widetilde{\boldsymbol{Z}}_i = (1, E_i, \mathrm{vec}(\boldsymbol{T}_i)^\top, \boldsymbol{Z}_i^\top)^\top$.

- **Step 9:** Update

$$O_i \mid \cdot \sim \begin{cases} N(\alpha_Y + \beta_{EY} E_i + \boldsymbol{\beta}_{TY}^\top \mathrm{vec}(\boldsymbol{T}_i) + \boldsymbol{\beta}_{ZY}^\top \boldsymbol{Z}_i, 1) \mathcal{I}[O_i > 0] & \text{if } Y_i = 1 \\ N(\alpha_Y + \beta_{EY} E_i + \boldsymbol{\beta}_{TY}^\top \mathrm{vec}(\boldsymbol{T}_i) + \boldsymbol{\beta}_{ZY}^\top \boldsymbol{Z}_i, 1) \mathcal{I}[O_i < 0] & \text{if } Y_i = 0. \end{cases}$$

# Web Appendix D An Alternative Two-step Method

Instead of estimating all model parameters jointly, an alternative approach is to use a two-step estimation method. Specifically, the first step is to use algorithm-based MPCA (Lu et al., 2008) on $\boldsymbol{X}_i$ to obtain latent features $\widehat{\boldsymbol{T}}_i^*$ and loadings $\widehat{\boldsymbol{A}}^*$ and $\widehat{\boldsymbol{B}}^*$, and second step is to fit a conventional linear regression model for (2) and a conventional probit model for (3) with extracted $\mathrm{vec}(\widehat{\boldsymbol{T}}_i^*)$, $E_i$, and $\boldsymbol{C}_i$, to obtain estimated model parameters $\widehat{\boldsymbol{\beta}}_{ET}^*$, $\widehat{\boldsymbol{\beta}}_{TY}^*$, and $\widehat{\boldsymbol{\Omega}}_{ZT}^*$ among others. We can then rotate the estimated $\widehat{\boldsymbol{A}}^*$, $\widehat{\boldsymbol{B}}^*$, $\widehat{\boldsymbol{\beta}}_{ET}^*$, $\widehat{\boldsymbol{\beta}}_{TY}^*$, and $\widehat{\boldsymbol{\Omega}}_{ZT}^*$ by Varimax principle, and finally use the Varimax rotated parameters and loadings to calculate the causal decomposition effects and to identify active indicators of mediation.

Two-step methods may lead to bias and could be less efficient than the joint modelling approach in general. This is because the two-step method estimates parameters using separate likelihoods, instead of considering a full likelihood for all parameters in the joint model, which ignores the information sharing between submodels. Jiang et al. (2020) compared the two approaches for estimating prediction parameters through simulation and found that the two-step method is less efficient than the joint modeling approach. We will compare the estimation efficiency of causal decomposition effects using these two methods in our simulation study.

# Web Appendix E   Implied observed data models

Based on the proposed joint model (1-3), we can derive two implied models: (i) Regressing each element of $\boldsymbol{X}_i$ on $E_i$ (instead of $\boldsymbol{T}_i$) and $\boldsymbol{Z}_i$; (ii) Regressing $Y_i$ on $\boldsymbol{X}_i$ (instead of $\boldsymbol{T}_i$), $E_i$, and $\boldsymbol{Z}_i$. To derive (i),

$$\begin{aligned} E[\text{vec}(\boldsymbol{X}_i) \mid E_i, \boldsymbol{Z}_i] &= E[E(\text{vec}(\boldsymbol{X}_i) \mid \boldsymbol{T}_i, E_i, \boldsymbol{Z}_i) \mid E_i, \boldsymbol{Z}_i] \\ &= \text{vec}(\boldsymbol{\mu}) + (\boldsymbol{B} \otimes \boldsymbol{A}) E[\text{vec}(\boldsymbol{T}_i) \mid E_i, \boldsymbol{Z}_i] \\ &= \text{vec}(\boldsymbol{\mu}) + (\boldsymbol{B} \otimes \boldsymbol{A})(\boldsymbol{\beta}_{ET} E_i + \boldsymbol{\Omega}_{ZT} \boldsymbol{Z}_i) \end{aligned}$$

and

$$\begin{aligned} \text{Var}[\text{vec}(\boldsymbol{X}_i) \mid E_i, \boldsymbol{Z}_i] &= E[\text{Var}(\text{vec}(\boldsymbol{X}_i) \mid \boldsymbol{T}_i, E_i, \boldsymbol{Z}_i) \mid E_i, \boldsymbol{Z}_i] + \text{Var}[E(\text{vec}(\boldsymbol{X}_i) \mid \boldsymbol{T}_i, E_i, \boldsymbol{Z}_i) \mid E_i, \boldsymbol{Z}_i] \\ &= E[\phi^{-1} \boldsymbol{I}_{pq} \mid E_i, \boldsymbol{Z}_i] + (\boldsymbol{B} \otimes \boldsymbol{A}) \text{Var}[\text{vec}(\boldsymbol{T}_i) \mid E_i, \boldsymbol{Z}_i] (\boldsymbol{B} \otimes \boldsymbol{A})^\top \\ &= \phi^{-1} \boldsymbol{I}_{pq} + (\boldsymbol{B} \otimes \boldsymbol{A}) \boldsymbol{I}_{p_0 q_0} (\boldsymbol{B} \otimes \boldsymbol{A})^\top \\ &= \phi^{-1} \boldsymbol{I}_{pq} + \boldsymbol{W} \boldsymbol{W}^\top, \end{aligned}$$

resulting in the first implied model

$$\text{vec}(\boldsymbol{X}_i) = \text{vec}(\boldsymbol{\mu}) + \boldsymbol{\beta}_{EX} E_i + \boldsymbol{\Omega}_{ZX} \boldsymbol{Z}_i + \text{vec}(\widetilde{\boldsymbol{\varepsilon}}_{X,i}), \tag{E.1}$$

where $\boldsymbol{W} = \boldsymbol{B} \otimes \boldsymbol{A}$, $\boldsymbol{\beta}_{EX} = \boldsymbol{W} \boldsymbol{\beta}_{ET}$, $\boldsymbol{\Omega}_{ZX} = \boldsymbol{W} \boldsymbol{\Omega}_{ZT}$, and $\text{vec}(\widetilde{\boldsymbol{\varepsilon}}_{X,i}) \sim N(\boldsymbol{0}, \phi^{-1} \boldsymbol{I}_{pq} + \boldsymbol{W} \boldsymbol{W}^\top)$. In the regression of the elements of $\boldsymbol{X}_i$ on $E_i$ and $\boldsymbol{Z}_i$, the new coefficients are the product of MPCA loadings and the original coefficients in the regression of $\boldsymbol{T}_i$ on $E_i$ and $\boldsymbol{Z}_i$ in the joint model component (2), respectively.

To derive (ii), we first have

$$\begin{aligned} & f(\text{vec}(\boldsymbol{T}_i) \mid \boldsymbol{X}_i, E_i, \boldsymbol{Z}_i) \propto f(\boldsymbol{X}_i \mid \boldsymbol{T}_i, E_i, \boldsymbol{Z}_i) f(\text{vec}(\boldsymbol{T}_i) \mid E_i, \boldsymbol{Z}_i) \\ & \propto \exp\left\{ -\frac{\phi}{2} \left\| \text{vec}(\boldsymbol{X}_i) - \text{vec}(\boldsymbol{\mu}) - (\boldsymbol{B} \otimes \boldsymbol{A}) \text{vec}(\boldsymbol{T}_i) \right\|_F^2 - \frac{1}{2} \left\| \text{vec}(\boldsymbol{T}_i) - \boldsymbol{\beta}_{ET} E_i - \boldsymbol{\Omega}_{ZT} \boldsymbol{Z}_i \right\|^2 \right\} \\ & \propto \exp\left\{ -\frac{1}{2} \left[ \text{vec}(\boldsymbol{T}_i)^\top \widetilde{\boldsymbol{C}}^{-1} \text{vec}(\boldsymbol{T}_i) - 2 \text{vec}(\boldsymbol{T}_i)^\top \widetilde{\boldsymbol{C}}^{-1} \widetilde{\boldsymbol{m}}_i \right] \right\} \\ & \propto \exp\left\{ -\frac{1}{2} \left[ \text{vec}(\boldsymbol{T}_i) - \widetilde{\boldsymbol{m}}_i \right]^\top \widetilde{\boldsymbol{C}}^{-1} \left[ \text{vec}(\boldsymbol{T}_i) - \widetilde{\boldsymbol{m}}_i \right] \right\}, \end{aligned} \tag{E.2}$$

where $\widetilde{\boldsymbol{C}} = (\phi(\boldsymbol{B} \otimes \boldsymbol{A})^\top (\boldsymbol{B} \otimes \boldsymbol{A}) + \boldsymbol{I}_{p_0 q_0})^{-1} = (\phi \boldsymbol{I}_{p_0 q_0} + \boldsymbol{I}_{p_0 q_0})^{-1} = (\phi + 1)^{-1} \boldsymbol{I}_{p_0 q_0}$, and $\widetilde{\boldsymbol{m}}_i = \widetilde{\boldsymbol{C}}[\boldsymbol{\beta}_{ET} E_i + \boldsymbol{\Omega}_{ZT} \boldsymbol{Z}_i + \phi(\boldsymbol{B} \otimes \boldsymbol{A})^\top (\text{vec}(\boldsymbol{X}_i) - \text{vec}(\boldsymbol{\mu}))]$. Equation (E.2) is proportional to a normal density, which indicates $\text{vec}\,(\boldsymbol{T}_i) \mid \boldsymbol{X}_i, E_i, \boldsymbol{Z}_i \sim N(\widetilde{\boldsymbol{m}}_i, \widetilde{\boldsymbol{C}})$.

Next, recall that a latent outcome $O_i$ was defined as $Y_i = \mathcal{I}(O_i > 0)$ in Web Appendix C, and we have $O_i \mid E_i, \boldsymbol{T}_i, \boldsymbol{Z}_i \sim N(\alpha_Y + \beta_{EY} E_i + \boldsymbol{\beta}_{TY}^\top \text{vec}(\boldsymbol{T}_i) + \boldsymbol{\beta}_{ZY}^\top \boldsymbol{Z}_i, 1)$. Then,

$$
\begin{aligned}
E[O_i \mid E_i, \boldsymbol{X}_i, \boldsymbol{Z}_i] &= E[E(O_i \mid \boldsymbol{T}_i, \boldsymbol{X}_i, E_i, \boldsymbol{Z}_i) \mid \boldsymbol{X}_i, E_i, \boldsymbol{Z}_i] \\
&= \alpha_Y + \beta_{EY} E_i + \boldsymbol{\beta}_{TY}^\top E[\text{vec}(\boldsymbol{T}_i) \mid \boldsymbol{X}_i, E_i, \boldsymbol{Z}_i] + \boldsymbol{\beta}_{ZY}^\top \boldsymbol{Z}_i \\
&= \alpha_Y + \beta_{EY} E_i + \boldsymbol{\beta}_{TY}^\top \widetilde{\boldsymbol{m}}_i + \boldsymbol{\beta}_{ZY}^\top \boldsymbol{Z}_i \quad \text{by (E.2)} \\
&= \left[\alpha_Y - (\phi+1)^{-1} \phi((\boldsymbol{B} \otimes \boldsymbol{A}) \boldsymbol{\beta}_{TY})^\top \text{vec}(\boldsymbol{\mu})\right] + \left[\beta_{EY} + (\phi+1)^{-1} \boldsymbol{\beta}_{ET}^\top \boldsymbol{\beta}_{TY}\right] E_i \\
&\quad + \left[\phi(\phi+1)^{-1}((\boldsymbol{B} \otimes \boldsymbol{A}) \boldsymbol{\beta}_{TY})^\top\right] \text{vec}(\boldsymbol{X}_i) + \left[\boldsymbol{\beta}_{ZY} + (\phi+1)^{-1} \boldsymbol{\Omega}_{ZT}^\top \boldsymbol{\beta}_{TY}\right]^\top \boldsymbol{Z}_i
\end{aligned} \tag{E.3}
$$

and

$$
\begin{aligned}
\text{Var}[O_i \mid E_i, \boldsymbol{X}_i, \boldsymbol{Z}_i] &= E[\text{Var}(O_i \mid \boldsymbol{T}_i, \boldsymbol{X}_i, E_i, \boldsymbol{Z}_i) \mid \boldsymbol{X}_i, E_i, \boldsymbol{Z}_i] + \text{Var}[E(O_i \mid \boldsymbol{T}_i, \boldsymbol{X}_i, E_i, \boldsymbol{Z}_i) \mid \boldsymbol{X}_i, E_i, \boldsymbol{Z}_i] \\
&= 1 + \boldsymbol{\beta}_{TY}^\top \text{Var}(\text{vec}(\boldsymbol{T}_i) \mid \boldsymbol{X}_i, E_i, \boldsymbol{Z}_i) \boldsymbol{\beta}_{TY} \\
&= 1 + (\phi+1)^{-1} \boldsymbol{\beta}_{TY}^\top \boldsymbol{\beta}_{TY} \quad \text{by (E.2)}.
\end{aligned} \tag{E.4}
$$

This indicates $O_i \mid E_i, \boldsymbol{X}_i, \boldsymbol{Z}_i \sim N(\boldsymbol{\mu}_{OX,i}, \boldsymbol{V}_{OX})$, where $\boldsymbol{\mu}_{OX,i} = E[O_i \mid E_i, \boldsymbol{X}_i, \boldsymbol{Z}_i]$ and $\boldsymbol{V}_{OX} = \text{Var}[O_i \mid E_i, \boldsymbol{X}_i, \boldsymbol{Z}_i]$, which gives $\Pr(Y_i = 1) = \Pr(O_i > 0) = \Phi(-\boldsymbol{V}_{OX}^{-1/2} \boldsymbol{\mu}_{OX,i})$.

Finally, the above suggests the second implied model

$$
\Phi^{-1}[\Pr(Y_i = 1 \mid E_i, \boldsymbol{X}_i, \boldsymbol{Z}_i)] = \alpha_Y^\dagger + \beta_{EY}^\dagger E_i + \boldsymbol{\beta}_{XY}^\top \text{vec}(\boldsymbol{X}_i) + \boldsymbol{\beta}_{ZY}^{\dagger\top} \boldsymbol{Z}_i, \tag{E.5}
$$

where

$$
\begin{aligned}
\alpha_Y^\dagger &= ((\phi+1)^{-1} \boldsymbol{\beta}_{TY}^\top \boldsymbol{\beta}_{TY} + 1)^{-1/2} \left[\alpha_Y - (\phi+1)^{-1} \phi(\boldsymbol{W} \boldsymbol{\beta}_{TY})^\top \text{vec}(\boldsymbol{\mu})\right] \\
\beta_{EY}^\dagger &= ((\phi+1)^{-1} \boldsymbol{\beta}_{TY}^\top \boldsymbol{\beta}_{TY} + 1)^{-1/2} \left[\beta_{EY} + (\phi+1)^{-1} \boldsymbol{\beta}_{ET}^\top \boldsymbol{\beta}_{TY}\right] \\
\boldsymbol{\beta}_{XY} &= ((\phi+1)^{-1} \boldsymbol{\beta}_{TY}^\top \boldsymbol{\beta}_{TY} + 1)^{-1/2} \left[\phi(\phi+1)^{-1} (\boldsymbol{W} \boldsymbol{\beta}_{TY})\right] \\
\boldsymbol{\beta}_{ZY}^\dagger &= ((\phi+1)^{-1} \boldsymbol{\beta}_{TY}^\top \boldsymbol{\beta}_{TY} + 1)^{-1/2} \left[\boldsymbol{\beta}_{ZY} + (\phi+1)^{-1} \boldsymbol{\Omega}_{ZT}^\top \boldsymbol{\beta}_{TY}\right].
\end{aligned}
$$

The second implied model suggests that the treatment effect $\beta_{EY}^\dagger$ and the covariate effect $\boldsymbol{\beta}_{ZY}^\dagger$ are constituted by two parts, from $E_i/\boldsymbol{Z}_i$ to $Y_i$ directly, and indirectly from $E_i/\boldsymbol{Z}_i$ to $\boldsymbol{T}_i$, then to $Y_i$. It also shows that the observed matrix-valued data effect $\boldsymbol{\beta}_{XY}$ is proportional to the product of MPCA loadings and the effect of latent features $\boldsymbol{T}_i$ on $Y_i$. The two implied models reflect the association structure between $Y_i$, $E_i$, $\boldsymbol{Z}_i$, and $\boldsymbol{X}_i$ marginal on $\boldsymbol{T}_i$. Based on the implied model, one could consider quantities such as $\beta_{EX,m} \beta_{XY,m}$ for $m = 1, \cdots, pq$, where $\beta_{EX,m}$ and $\beta_{XY,m}$ are the $m$th element of $\boldsymbol{\beta}_{EX}$ and $\boldsymbol{\beta}_{XY}$, respectively, which would quantify mediation in a model where $\boldsymbol{X}_i$ is the true causal mediator. However, under the latent variable mediation model, such quantities would not generally correspond to causal effects, and in particular, are different from the quantities (4) we used to quantify

mediation. Simulated comparisons between these measures might be of interest, especially under scenarios where the real data does not follow the latent variable mediation model, but where such a model is anyway used for regularization/dimension reduction purposes. This is left as further work.

# Web Appendix F Identifiability

## F.1 Identifiability of Model Parameters

Here we show that the joint model parameters $\boldsymbol{\mu}$, $\alpha_Y$, $\beta_{EY}$, $\boldsymbol{\beta}_{ZY}$ and $\phi$ are identifiable, and $\boldsymbol{A}$, $\boldsymbol{B}$, $\boldsymbol{\beta}_{ET}$, $\boldsymbol{\beta}_{TY}$, $\boldsymbol{\Omega}_{ZT}$ are identifiable up to orthogonal rotations, following a similar proof given in the Web Appendix D of Derkach et al. (2019). Let $\Theta^1 = (\boldsymbol{A}^1, \boldsymbol{B}^1, \boldsymbol{\mu}^1, \boldsymbol{\beta}^1_{ET}, \boldsymbol{\Omega}^1_{ZT}, \alpha^1_Y, \beta^1_{EY}, \boldsymbol{\beta}^1_{TY}, \boldsymbol{\beta}^1_{ZY}, \phi^1)$ and $\Theta^2 = (\boldsymbol{A}^2, \boldsymbol{B}^2, \boldsymbol{\mu}^2, \boldsymbol{\beta}^2_{ET}, \boldsymbol{\Omega}^2_{ZT}, \alpha^2_Y, \beta^2_{EY}, \boldsymbol{\beta}^2_{TY}, \boldsymbol{\beta}^2_{ZY}, \phi^2)$ denote any two sets of parameters in the joint model, and let $\boldsymbol{P} \in \mathbb{R}^{p_0 \times p_0}$ and $\boldsymbol{Q} \in \mathbb{R}^{q_0 \times q_0}$ denote any orthogonal rotation matrices such that $\boldsymbol{P}^\top \boldsymbol{P} = \boldsymbol{P}\boldsymbol{P}^\top = \boldsymbol{I}_{p_0}$ and $\boldsymbol{Q}^\top \boldsymbol{Q} = \boldsymbol{Q}\boldsymbol{Q}^\top = \boldsymbol{I}_{q_0}$. We show that if $f(Y_i, \boldsymbol{X}_i \mid E_i, \boldsymbol{Z}_i; \Theta^1) = f(Y_i, \boldsymbol{X}_i \mid E_i, \boldsymbol{Z}_i; \Theta^2)$ for all values of $Y_i, E_i, \boldsymbol{X}_i$, we have $\boldsymbol{A}^1 = \boldsymbol{A}^2\boldsymbol{P}$, $\boldsymbol{B}^1 = \boldsymbol{B}^2\boldsymbol{Q}$, $\boldsymbol{\mu}^1 = \boldsymbol{\mu}^2$, $\boldsymbol{\beta}^1_{ET} = (\boldsymbol{Q} \otimes \boldsymbol{P})^\top \boldsymbol{\beta}^2_{ET}$, $\boldsymbol{\Omega}^1_{ZT} = (\boldsymbol{Q} \otimes \boldsymbol{P})^\top \boldsymbol{\Omega}^2_{ZT}$, $\alpha^1_Y = \alpha^2_Y$, $\beta^1_{EY} = \beta^2_{EY}$, $\boldsymbol{\beta}^1_{TY} = (\boldsymbol{Q} \otimes \boldsymbol{P})^\top \boldsymbol{\beta}^2_{TY}$, $\boldsymbol{\beta}^1_{ZY} = \boldsymbol{\beta}^2_{ZY}$, and $\phi^1 = \phi^2$.

The conditional joint density function $f(Y_i, \boldsymbol{X}_i \mid E_i, \boldsymbol{Z}_i; \Theta)$ (denoted by $f(\cdot; \Theta)$ in short) can be decomposed into

$$f(Y_i, \boldsymbol{X}_i \mid E_i, \boldsymbol{Z}_i; \Theta) = f(Y_i \mid \boldsymbol{X}_i, E_i, \boldsymbol{Z}_i; \Theta) f(\boldsymbol{X}_i \mid E_i, \boldsymbol{Z}_i; \boldsymbol{A}, \boldsymbol{B}, \boldsymbol{\beta}_{ET}, \boldsymbol{\Omega}_{ZT}, \phi). \tag{F.1}$$

If $f(\cdot; \Theta^1) = f(\cdot; \Theta^2)$, then $f(\boldsymbol{X}_i \mid E_i, \boldsymbol{Z}_i; \boldsymbol{A}^1, \boldsymbol{B}^1, \boldsymbol{\beta}^1_{ET}, \boldsymbol{\Omega}^1_{ZT}, \phi^1) = f(\boldsymbol{X}_i \mid E_i, \boldsymbol{Z}_i; \boldsymbol{A}^2, \boldsymbol{B}^2, \boldsymbol{\beta}^2_{ET}, \boldsymbol{\Omega}^2_{ZT}, \phi^2)$. From equation (E.1), we have $\mathrm{vec}(\boldsymbol{X}_i) \mid (E_i, Z_i) \sim N(\mathrm{vec}(\boldsymbol{\mu}) + \boldsymbol{W}\boldsymbol{\beta}_{ET}E_i + \boldsymbol{W}\boldsymbol{\Omega}_{ZT}\boldsymbol{Z}_i, \phi^{-1}\boldsymbol{I}_{pq} + \boldsymbol{W}\boldsymbol{W}^\top)$, where $\boldsymbol{W} = \boldsymbol{B} \otimes \boldsymbol{A}$. Note that $\phi^{-1}\boldsymbol{I}_{pq} + \boldsymbol{W}\boldsymbol{W}^\top$ is the variance of the factor analysis model in Anderson and Rubin (1956), with the additional constraint that the residual variance only depends on a single parameter $\phi$. Based on the sufficient condition 1 (Theorem 5.1) in Anderson and Rubin (1956) under some mild conditions, we have $\phi^1 = \phi^2$ and $\boldsymbol{W}$ identifiable up to rotation by an orthonormal matrix $\boldsymbol{R} \in \mathbb{R}^{p_0q_0 \times p_0q_0}$ (i.e. $\boldsymbol{W}^1 = \boldsymbol{W}^2\boldsymbol{R}$).

Furthermore, we have

$$f(\boldsymbol{X}_i \mid E_i, \boldsymbol{Z}_i; \boldsymbol{A}, \boldsymbol{B}, \boldsymbol{\beta}_{ET}, \boldsymbol{\Omega}_{ZT}, \phi) = \int_{\boldsymbol{t}} f(\boldsymbol{X}_i \mid \boldsymbol{t}; \boldsymbol{A}, \boldsymbol{B}, \phi) f(\boldsymbol{t} \mid E_i, \boldsymbol{Z}_i; \boldsymbol{\beta}_{ET}, \boldsymbol{\Omega}_{ZT}) d\boldsymbol{t}.$$

Note that $f(\boldsymbol{X}_i \mid \boldsymbol{T}_i; \boldsymbol{A}, \boldsymbol{B}, \phi)$ is the density function of a probabilistic MPCA model (Equation (1) in the main text). The identifiability of Equation (1) is discussed in Hung et al. (2012) and Ding and Cook (2014), the latter referring to it by the name of "dimension folding PCA". Hung et al. (2012) refer to earlier theorems from Li et al. (2010) for existence and uniqueness of the Kronecker envelope, that is, the subspace $\mathrm{Span}(\boldsymbol{B} \otimes \boldsymbol{A})$. If the Kronecker envelope is identifiable, $\mathrm{Span}(\boldsymbol{A})$ and $\mathrm{Span}(\boldsymbol{B})$ are also identifiable (as claimed by Ding and Cook, 2014), because orthonormal matrices with fixed dimension $\boldsymbol{A}$ and $\boldsymbol{B}$ can be reverse calculated from $\boldsymbol{B} \otimes \boldsymbol{A}$ (generally this would only work up to a division/multiplication by a constant, but here the scale of $\boldsymbol{A}$ and $\boldsymbol{B}$ is fixed). To

demonstrate rotational invariance, we note that if we have $\boldsymbol{A}^1 = \boldsymbol{A}^2\boldsymbol{P}$, $\boldsymbol{B}^1 = \boldsymbol{B}^2\boldsymbol{Q}$, and $\boldsymbol{T}_i^1 = \boldsymbol{P}^{-1}\boldsymbol{T}_i^2(\boldsymbol{Q}^\top)^{-1}$, where $\boldsymbol{P}$ and $\boldsymbol{Q}$ are any nonsingular matrices, submodel (1) remains the same. However, to preserve the properties of the model, $\boldsymbol{A}$ and $\boldsymbol{B}$ have to be orthonormal, and to ensure this, we require $\boldsymbol{P}$ and $\boldsymbol{Q}$ to be be orthonormal. To see this, $(\boldsymbol{A}^1)^\top\boldsymbol{A}^1 = \boldsymbol{P}^\top(\boldsymbol{A}^2)^\top\boldsymbol{A}^2\boldsymbol{P}^\top = \boldsymbol{P}^\top\boldsymbol{P} = \boldsymbol{I}_{p_0}$ and $(\boldsymbol{B}^1)^\top\boldsymbol{B}^1 = \boldsymbol{Q}^\top(\boldsymbol{B}^2)^\top\boldsymbol{B}^2\boldsymbol{Q}^\top = \boldsymbol{Q}^\top\boldsymbol{Q} = \boldsymbol{I}_{q_0}$. Thus, $\boldsymbol{A}$ and $\boldsymbol{B}$ are identifiable up to (but not including) orthogonal rotations. Subsequently, since $\boldsymbol{W}^1 = \boldsymbol{B}^1 \otimes \boldsymbol{A}^1 = (\boldsymbol{B}^2\boldsymbol{Q}) \otimes (\boldsymbol{A}^2\boldsymbol{P}) = (\boldsymbol{B}^2 \otimes \boldsymbol{A}^2)(\boldsymbol{Q} \otimes \boldsymbol{P}) = \boldsymbol{W}^2(\boldsymbol{Q} \otimes \boldsymbol{P})$, we have $\boldsymbol{R} = \boldsymbol{Q} \otimes \boldsymbol{P}$.

To identify $\boldsymbol{\mu}$, $\boldsymbol{\beta}_{ET}$ and $\boldsymbol{\Omega}_{ZT}$, from (E.1), we have $E(\text{vec}(\boldsymbol{X}_i) \mid E_i, \boldsymbol{Z}_i) = \text{vec}(\boldsymbol{\mu}) + (\boldsymbol{W}\boldsymbol{\beta}_{ET})E_i + (\boldsymbol{W}\boldsymbol{\Omega}_{ZT})\boldsymbol{Z}_i$, which implies $\boldsymbol{\mu}^1 = \boldsymbol{\mu}^2$, $\boldsymbol{W}^1\boldsymbol{\beta}_{ET}^1 = \boldsymbol{W}^2\boldsymbol{\beta}_{ET}^2$, and $\boldsymbol{W}^1\boldsymbol{\Omega}_{ZT}^1 = \boldsymbol{W}^2\boldsymbol{\Omega}_{ZT}^2$ for any values of $E_i$ and $\boldsymbol{Z}_i$. Since $\boldsymbol{W}^1 = \boldsymbol{W}^2(\boldsymbol{Q}\otimes\boldsymbol{P})$, we have $\boldsymbol{\beta}_{ET}^1 = (\boldsymbol{Q}\otimes\boldsymbol{P})^\top\boldsymbol{\beta}_{ET}^2$ and $\boldsymbol{\Omega}_{ZT}^1 = (\boldsymbol{Q} \otimes \boldsymbol{P})^\top\boldsymbol{\beta}_{ET}^2$.

For the identifiability of $\alpha_Y$, $\beta_{EY}$, $\boldsymbol{\beta}_{ZY}$ and $\boldsymbol{\beta}_{TY}$, we consider equation (F.1) again. If $f(\cdot;\Theta^1) = f(\cdot;\Theta^2)$, then $f(Y_i \mid \boldsymbol{X}_i, E_i, \boldsymbol{Z}_i; \Theta^1) = f(Y_i \mid \boldsymbol{X}_i, E_i, \boldsymbol{Z}_i; \Theta^2)$. Recall that we introduced a latent outcome variable $O_i$, such that $Y_i = \mathcal{I}(O_i > 0)$ in Web Appendix C, and we note that

$$f(Y_i \mid \boldsymbol{X}_i, E_i, \boldsymbol{Z}_i; \Theta) = \int_{o_i} f(Y_i \mid o_i) f(o_i \mid \boldsymbol{X}_i, E_i, \boldsymbol{Z}_i; \Theta) do_i.$$

From (E.3) and (E.4), we have $O_i \mid E_i, \boldsymbol{X}_i, \boldsymbol{Z}_i \sim N(\boldsymbol{\mu}_{OX,i}, \boldsymbol{V}_{OX})$, where

$$\begin{aligned}\boldsymbol{\mu}_{OX,i} = &\left[\alpha_Y - (\phi+1)^{-1}\phi(\boldsymbol{W}\boldsymbol{\beta}_{TY})^\top\text{vec}(\boldsymbol{\mu})\right] + \left[\beta_{EY} + (\phi+1)^{-1}\boldsymbol{\beta}_{ET}^\top\boldsymbol{\beta}_{TY}\right]E_i \\ &+ \left[\phi(\phi+1)^{-1}(\boldsymbol{W}\boldsymbol{\beta}_{TY})^\top\right]\text{vec}(\boldsymbol{X}_i) + \left[\boldsymbol{\beta}_{ZY} + (\phi+1)^{-1}\boldsymbol{\Omega}_{ZT}^\top\boldsymbol{\beta}_{TY}\right]^\top\boldsymbol{Z}_i\end{aligned}$$

and $\boldsymbol{V}_{OX} = 1+(\phi+1)^{-1}\boldsymbol{\beta}_{TY}^\top\boldsymbol{\beta}_{TY}$. This formulates a linear model for $O_i$ with covariates $E_i$, $\boldsymbol{X}_i$ and $\boldsymbol{Z}_i$. For any values of $E_i$, $\boldsymbol{X}_i$ and $\boldsymbol{Z}_i$, we have $\phi^1(\phi^1+1)^{-1}\boldsymbol{W}^1\boldsymbol{\beta}_{TY}^1 = \phi^2(\phi^2+1)^{-1}\boldsymbol{W}^2\boldsymbol{\beta}_{TY}^2$. Since $\phi^1 = \phi^2$, and $\boldsymbol{W}^1 = \boldsymbol{W}^2(\boldsymbol{Q} \otimes \boldsymbol{P})$, we have $\boldsymbol{\beta}_{TY}^1 = (\boldsymbol{Q} \otimes \boldsymbol{P})^\top\boldsymbol{\beta}_{TY}^2$. Similarly, we have $\boldsymbol{\beta}_{ZY}^1 = (\boldsymbol{Q} \otimes \boldsymbol{P})^\top\boldsymbol{\beta}_{ZY}^2$, $\alpha_Y^1 = \alpha_Y^2$, $\beta_{EY}^1 = \beta_{EY}^2$. Therefore, our joint model parameters $\boldsymbol{\mu}$, $\alpha_Y$, $\beta_{EY}$, $\boldsymbol{\beta}_{ZY}$ and $\phi$ are identifiable, and $\boldsymbol{A}$, $\boldsymbol{B}$, $\boldsymbol{\beta}_{ET}$, $\boldsymbol{\beta}_{TY}$, $\boldsymbol{\Omega}_{ZT}$ are identifiable up to orthogonal rotations.

## F.2 Identifiability of causal decomposition effects

To prove that overall NIE, NDE and TE are identifiable, we only need to prove $E[Y_i(e^*, T_i^1(e^*), \cdots, T_i^{p_0q_0}(e^*))]$, $E[Y_i(e^*, T_i^1(e), \cdots, T_i^{p_0q_0}(e))]$, and $E[Y_i(e, T_i^1(e), \cdots, T_i^{p_0q_0}(e))]$ are identifiable. Below we present the derivations of identifiability for $E[Y_i(e^*, T_i^1(e), \cdots, T_i^{p_0q_0}(e))]$ as an example: Let $\boldsymbol{t}^\dagger = \boldsymbol{\beta}_{TY}^\top\boldsymbol{t}$ and $\text{vec}(\boldsymbol{T}_i^\dagger) = \boldsymbol{\beta}_{TY}^\top\text{vec}(\boldsymbol{T}_i)$. Substituting $(e^0, e^1, \cdots, e^{p_0q_0}) = (e^*, e, \cdots, e)$ into Equation (B.5) in the main text, and then use integration by substitution

$$\begin{aligned}&E[Y_i(e^*, T_i^1(e), \cdots, T_i^{p_0q_0}(e))] \\ &= E_{\boldsymbol{Z}_i}\left\{\int_{\boldsymbol{t}} \Phi(\alpha_Y + \beta_{EY}e^* + \boldsymbol{\beta}_{TY}^\top\boldsymbol{t} + \boldsymbol{\beta}_{ZY}^\top\boldsymbol{Z}_i) f_{T_i^1|E_i=e,\boldsymbol{Z}_i}(t^1)\cdots f_{T_i^{p_0q_0}|E_i=e,\boldsymbol{Z}_i}(t^{p_0q_0})\mathrm{d}\boldsymbol{t}\right\} \\ &= E_{\boldsymbol{Z}_i}\left\{\int_{\boldsymbol{t}} \Phi(\alpha_Y + \beta_{EY}e^* + \boldsymbol{\beta}_{TY}^\top\boldsymbol{t} + \boldsymbol{\beta}_{ZY}^\top\boldsymbol{Z}_i) f_{\text{vec}(\boldsymbol{T}_i)|E_i=e,\boldsymbol{Z}_i}(\boldsymbol{t})\mathrm{d}\boldsymbol{t}\right\}\end{aligned}$$

$$= E_{\boldsymbol{Z}_i}\left\{\int_{\boldsymbol{t}^\dagger}\Phi(\alpha_Y+\beta_{EY}e^*+\boldsymbol{t}^\dagger+\boldsymbol{\beta}_{ZY}^\top\boldsymbol{Z}_i)\mathrm{d}F_{\mathrm{vec}(\boldsymbol{T}_i^\dagger)|E_i=e,\boldsymbol{Z}_i}(\boldsymbol{t}^\dagger)\right\}, \tag{F.2}$$

where $F_{\mathrm{vec}(\boldsymbol{T}_i^\dagger)|E_i=e,\boldsymbol{Z}_i}(\boldsymbol{t}^\dagger)$ is the conditional cumulative density function of $\boldsymbol{\beta}_{TY}^\top\mathrm{vec}(\boldsymbol{T}_i)\mid E_i = e, \boldsymbol{Z}_i$, which follows $N(\boldsymbol{\beta}_{TY}^\top\boldsymbol{\beta}_{ET}e+\boldsymbol{\beta}_{TY}^\top\boldsymbol{\Omega}_{ZT}\boldsymbol{z},\boldsymbol{\beta}_{TY}^\top\boldsymbol{\beta}_{TY})$ by model (2). Since $\alpha_Y$, $\beta_{EY}$, $\boldsymbol{\beta}_{ZY}$, $\boldsymbol{\beta}_{TY}^\top\boldsymbol{\Omega}_{ZT}$, $\boldsymbol{\beta}_{ET}^\top\boldsymbol{\beta}_{TY}$, and $\boldsymbol{\beta}_{TY}^\top\boldsymbol{\beta}_{TY}$ are all identifiable, $E[Y_i(e^*,T_i^1(e),\cdots,T_i^{p_0q_0}(e))]$ is identifiable.

We note that individual indirect pathways $\mathrm{NIE}_1$ to $\mathrm{NIE}_{p_0q_0}$ are only identifiable up to any orthogonal rotation. This is because $\boldsymbol{\beta}_{TY}^\top(T_i^1(e^1),\cdots,T_i^{p_0q_0}(e^{p_0q_0}))^\top\mid\boldsymbol{Z}_i$ follows $N(\sum_{j=1}^{p_0q_0}\beta_{TY,j}\beta_{ET,j}e^j+\boldsymbol{\beta}_{TY}^\top\boldsymbol{\Omega}_{ZT}\boldsymbol{Z}_i,\boldsymbol{\beta}_{TY}^\top\boldsymbol{\beta}_{TY})$ in general, and indirect individual pathway biproducts $\beta_{ET,j}\beta_{TY,j}$ for $j=1,\cdots,p_0q_0$ are only identifiable up to any orthogonal rotation.

# Web Appendix G Additional Comparative Simulation Study

## G.1 Joint and Two-step PCA model

Here we include additional comparisons to alternative models to further illustrate the performance of the proposed joint MPCA model. As previous literature has proposed PCA-based methods for high-dimensional mediation analysis, the most natural comparison is to a joint model that is otherwise similar to the proposed one, but uses probabilistic PCA (Tipping and Bishop, 1999) parametrization instead of the MPCA parametrization. As discussed in *Remark 1* in the main text, the two models can be understood as nested, where the unrestricted PCA model does not impose the Kronecker envelope constraint to the loading matrices, and thus does not make use of the row and column information in the matrix valued data, resulting in a larger number of free parameters to be estimated.

The formulation of a three-component joint PCA model is the similar to the proposed joint MPCA model (1-3), with the submodel (1) modified to

$$\mathrm{vec}(\boldsymbol{X}_i)=\mathrm{vec}(\boldsymbol{\mu})+\boldsymbol{\Lambda}\mathrm{vec}(\boldsymbol{T}_i)+\mathrm{vec}(\boldsymbol{\varepsilon}_{X,i}), \tag{G.1}$$

where $\boldsymbol{\Lambda}\in\mathbb{R}^{pq\times p_0q_0}$ is unconstrained compared to the MPCA formulation. We use a similar Gibbs sampling algorithm for estimation, and the complete updating algorithm is similar to Steps 1-9 given in Web Appendix C for the joint MPCA model. The only difference is to replace the Steps 1 and 2 for updating $\boldsymbol{A}$ and $\boldsymbol{B}$ with a single step to update $\boldsymbol{\Lambda}$, which is

- **Step 1:** Update $\boldsymbol{\Lambda}_{[,j]}\mid\cdot\overset{\mathrm{d}}{=}\boldsymbol{N}_{\Lambda_{[,-j]}}\widetilde{\boldsymbol{a}}_j$ for $j=1,...,p_0q_0$. $\widetilde{\boldsymbol{a}}_j\sim\mathrm{vMF}(\phi\boldsymbol{N}_{\Lambda_{[,-j]}}^\top\sum_{i=1}^n T_i^j\mathrm{vec}(\boldsymbol{X}_i)^{-j})$, where $\mathrm{vec}(\boldsymbol{X}_i)^{-j}=\mathrm{vec}(\boldsymbol{X}_i)-\mathrm{vec}(\boldsymbol{\mu})-\boldsymbol{\Lambda}_{[,-j]}\mathrm{vec}(\boldsymbol{T}_i)_{[-j]}$, $\boldsymbol{\Lambda}_{[,j]}$ and $\boldsymbol{\Lambda}_{[,-j]}$ represent the $j$th column of $\boldsymbol{\Lambda}$ and $\boldsymbol{\Lambda}$ with its $j$th column removed, respectively. $\mathrm{vec}(\boldsymbol{T}_i)_{[-j]}$ represents $\mathrm{vec}(\boldsymbol{T}_i)$ with its $j$th element (i.e. $T_i^j$) removed.

For completeness, we also included the corresponding two-step PCA model, where the first step is to use algorithm-based PCA to estimate loadings $\widehat{\boldsymbol{\Lambda}}$, and the second step is to fit the linear submodel (2) and the probit submodel (3).

## G.2 Simulation Setting

We considered 6 different models/estimation methods: (1) joint MPCA model with a weakly-informative prior, (2) joint PCA model with a weakly-informative prior, (3) joint MPCA model with a non-informative prior, (4) joint PCA model with a non-informative prior, (5) two-step MPCA model, and (6) two-step PCA model. A weakly-informative prior (denoted by WI) is defined as $\alpha_Y \sim \beta_{EY} \sim N(0, 1)$, $\boldsymbol{\beta}_{ET} \sim \boldsymbol{\beta}_{TY} \sim N(\mathbf{0}, \boldsymbol{I}_{p_0q_0})$, and a non-informative prior (denoted by NI) is defined as $\alpha_Y \sim \beta_{EY} \sim N(0, 10)$, $\boldsymbol{\beta}_{ET} \sim \boldsymbol{\beta}_{TY} \sim N(\mathbf{0}, 10\boldsymbol{I}_{p_0q_0})$. The data generation procedure and other parameter settings are the same as that in Section 3.1 in the main text, with exceptions that here we only consider the dimension $(p, q) = (10, 10)$ for the matrix-valued data. Similarly, $(p_0, q_0)$ is fixed at $(2, 2)$ across all scenarios.

## G.3 Results

Web Table G.1: Comparison between different models

| ***n*** | **Effects** | **MSE**[1] | **Var**[1] | **Bias**[1] | **Estimate**[2] | **MSE**[1] | **Var**[1] | **Bias**[1] | **Estimate**[2] |
|---|---|---|---|---|---|---|---|---|---|
| | | **Joint Model: MPCA, WI** | | | | **Joint Model: PCA, WI** | | | |
| | NIE | 1.878 | 1.861 | -4.512 | 0.0886 | 1.874 | 1.857 | -4.620 | 0.0885 |
| 100 | NDE | 5.846 | 5.842 | -3.997 | 0.0804 | 5.852 | 5.850 | -3.723 | 0.0807 |
| | TE | 6.337 | 6.277 | -8.509 | 0.1690 | 6.342 | 6.285 | -8.343 | 0.1692 |
| | NIE | 0.643 | 0.644 | -0.882 | 0.0922 | 0.646 | 0.646 | -0.910 | 0.0922 |
| 300 | NDE | 1.929 | 1.930 | -1.763 | 0.0826 | 1.931 | 1.932 | -1.721 | 0.0827 |
| | TE | 1.958 | 1.954 | -2.645 | 0.1749 | 1.957 | 1.954 | -2.631 | 0.1749 |
| | | **Joint Model: MPCA, NI** | | | | **Joint Model: PCA, NI** | | | |
| | NIE | 2.049 | 2.051 | -1.537 | 0.0916 | 2.060 | 2.062 | -1.600 | 0.0915 |
| 100 | NDE | 7.323 | 7.337 | 0.611 | 0.0850 | 7.292 | 7.307 | 0.615 | 0.0850 |
| | TE | 7.411 | 7.425 | -0.926 | 0.1766 | 7.394 | 7.407 | -0.985 | 0.1765 |
| | NIE | 0.659 | 0.660 | 0.089 | 0.0932 | 0.663 | 0.665 | 0.042 | 0.0931 |
| 300 | NDE | 2.086 | 2.091 | -0.220 | 0.0842 | 2.086 | 2.090 | -0.207 | 0.0842 |
| | TE | 2.069 | 2.073 | -0.131 | 0.1774 | 2.075 | 2.079 | -0.165 | 0.1773 |
| | | **Two-step: MPCA** | | | | **Two-step: PCA** | | | |
| | NIE | 3.415 | 3.416 | -2.319 | 0.0908 | 3.491 | 3.493 | -2.051 | 0.0911 |
| 100 | NDE | 7.900 | 7.856 | 7.689 | 0.0921 | 8.044 | 7.983 | 8.773 | 0.0932 |
| | TE | 9.175 | 9.164 | 5.371 | 0.1829 | 9.272 | 9.246 | 6.721 | 0.1842 |
| | NIE | 1.125 | 1.119 | -2.856 | 0.0902 | 1.097 | 1.092 | -2.621 | 0.0905 |
| 300 | NDE | 2.161 | 2.139 | 5.139 | 0.0895 | 2.169 | 2.144 | 5.409 | 0.0898 |
| | TE | 2.523 | 2.523 | 2.284 | 0.1798 | 2.515 | 2.512 | 2.787 | 0.1803 |

[1] The values displayed for MSE, bias, and variance are the actual values × 1000; MSE = Mean Squared Error; Var = Variance

[2] True NIE = 0.0931; True NDE = 0.0844; True TE = 0.1775

Web Table G.1 show the performance in estimating causal decomposition effects between these 6 methods. No clear difference was observed between joint MPCA versus joint PCA

using either weakly-informative prior and non-informative prior, as well as between two-step MPCA versus two-step PCA. This is within expected because MPCA and PCA can be considered nested models, and adding more parameters does not necessarily provide more estimation accuracy. Given the similar estimation performance, we emphasize that the joint MPCA model almost halve the computation time than the joint PCA model, due to a greatly reduced number of parameters being estimated, which provides a significant computational advantage.

Comparing different priors, for both joint MPCA and joint PCA models, weakly informative priors give smaller MSEs and variances than non-informative priors, while having slightly larger biases. These biases appear to converge towards 0 and are similar to or smaller than the two-step method when increasing sample size to 300. We note that both joint MPCA and joint PCA (using whichever priors) generally perform better than the corresponding two-step MPCA and two-step PCA, which again suggests the advantage of estimating parameters using a joint likelihood instead of two separate steps.

Figure G.1 shows scatter plots of the estimated mediation quantities versus true mediation quantities for the6 methods for small and large sample sizes. Comparing joint MPCA (Panel A1/A2) versus joint PCA (Panel B1/B2), we observe that joint PCA gives larger estimates for inactive indicators (bottom left red dots deviate more from 0 in B1/B2 panels than those in A1/A2 panels) in the small sample size setting ($n = 100$). This suggests the joint PCA model results in more noise than the joint MPCA model when identifying active indicators, especially in the small sample size setting. Increasing the sample size to $n = 300$ reduces these differences between joint PCA and joint MPCA, and both models' active indicators of mediation appear to converge towards their true values, and inactive indicators towards 0. For both MPCA and PCA, in the small sample size setting, the two-step methods (Panel A3/B3) have longer blue error bars than the corresponding joint models with weakly-informative priors (Panel A1/B1), which suggests that two-step methods have larger estimation variance for active indicators. Although the two-step methods seem to have smaller biases for active indicators, they do not converge towards the true mediation quantities when increasing the sample size to $n = 300$ (while joint models do converge), which suggests that the two-step method might not be a valid method in large samples.

Figure G.2 shows the heatmaps of the estimated mediation quantities with black dots indicating the simulated true indicators of mediation. For both joint models with weakly informative priors and non-informative priors, as well as the two-step method, PCA shows more noise than MPCA (deeper pink color for PCA), especially in the inactive indicator areas where there are no active indicators in the same row or column. This indicates an advantage of MPCA over PCA, which is to extract the feature from both rows and columns, so the areas of inactive indicators which are not in the same row or column of active indicators are not affected by feature extraction, resulting in a reduced noise. Instead, PCA-based method ignores the matrix structure and extracts features from mixed information of row and columns, so the model treats the inactive indicator area equally (i.e. do not distinguish if there are active indicators in the same row or column), which produces more noise.

In summary, the primary advantage of the proposed joint MPCA model over the PCA model is that it can reduce the noise in identifying inactive indicators of mediation. Also, it can greatly reduce the computation time due the more parsimonious specification, and provide more clear identification of active indicators of mediation.

# Web Appendix H Additional Model Misspecification Simulation Study

Web Table H.1: Model Misspecification

| $n$ | Effects | MSE[1] | Var[1] | Bias[1] | Estimate[2] | MSE[1] | Var[1] | Bias[1] | Estimate[2] |
|---|---|---|---|---|---|---|---|---|---|
| | | $(p_0, q_0) = (2, 2)$ | | | | $(p_0, q_0) = (2, 3)$ | | | |
| 100 | NIE | 1.878 | 1.861 | -4.512 | 0.0886 | 1.733 | 1.436 | -17.300 | 0.0758 |
| | NDE | 5.846 | 5.842 | -3.997 | 0.0804 | 4.402 | 4.105 | -17.465 | 0.0669 |
| | TE | 6.337 | 6.277 | -8.509 | 0.1690 | 5.726 | 4.526 | -34.765 | 0.1427 |
| 300 | NIE | 0.643 | 0.644 | -0.882 | 0.0922 | 0.643 | 0.556 | -9.420 | 0.0837 |
| | NDE | 1.929 | 1.930 | -1.763 | 0.0826 | 1.699 | 1.600 | -10.115 | 0.0743 |
| | TE | 1.958 | 1.954 | -2.645 | 0.1749 | 2.060 | 1.682 | -19.535 | 0.1580 |
| | | $(p_0, q_0) = (3, 2)$ | | | | $(p_0, q_0) = (3, 3)$ | | | |
| 100 | NIE | 1.716 | 1.428 | -17.049 | 0.0761 | 1.892 | 1.090 | -28.360 | 0.0647 |
| | NDE | 4.441 | 4.152 | -17.245 | 0.0672 | 3.749 | 2.909 | -29.082 | 0.0553 |
| | TE | 5.713 | 4.546 | -34.294 | 0.1432 | 6.561 | 3.268 | -57.442 | 0.1201 |
| 300 | NIE | 0.645 | 0.556 | -9.491 | 0.0836 | 0.823 | 0.458 | -19.132 | 0.0740 |
| | NDE | 1.663 | 1.565 | -10.076 | 0.0743 | 1.572 | 1.200 | -19.356 | 0.0650 |
| | TE | 2.049 | 1.669 | -19.567 | 0.1579 | 2.799 | 1.320 | -38.488 | 0.1390 |

[1] The values displayed for MSE, bias, and variance are the actual values × 1000; MSE = Mean Squared Error; Var = Variance
[2] True NIE = 0.0931; True NDE = 0.0844; True TE = 0.1775

## H.1 Simulation Setting

Here we provide an additional model misspecification study to further illustrate the estimation and identification performance of the proposed joint model. Similar to Section 3.1 in the main text, we simulate the true latent features assuming $(p_0, q_0) = (2, 2)$, but consider 4 different overspecified models when fitting the joint model: $(p_0, q_0) = (2, 2)$, $(2, 3)$, $(3, 2)$, and $(3, 3)$. Data generation procedure and all other parameter settings are chosen the same as those in Section 3.1.

## H.2 Results

Web Table H.1 shows the estimation performance of the causal decomposition effects when the model is misspecified (overspecified). Compared to the correctly specified model $(p_0, q_0) = (2, 2)$, incorrectly specified models have larger biases, but smaller variances for all decomposition effects. This suggests a bias-variance trade-off: with increased number of parameters, the biases increase, and the variances decrease. Increasing the sample size reduces the biases and variances.

Web Figure H.1 presents the scatter plots of the estimated mediation quantities versus true mediation quantities. In the small sample size setting, incorrectly specified models show

larger biases for the mediation indicators (red dots are more deviated from the black diagonal line) and larger variances from inactive indicators (bottom left red dots are more scattered) compared to the correctly specified model $(p_0, q_0) = (2, 2)$. However, when the sample size increases, the red dots move closer to the black diagonal line, and the bottom left red dots become more dense and closer to 0. This suggests that the incorrectly specified models are still converging to the true quantities, but slower than the correctly specified model, due to the unnecessarily increased number of parameters.

Web Figure H.2 presents heatmaps of the estimated mediation quantities for these 4 models. Compared to the correctly specified model $(p_0, q_0) = (2, 2)$, incorrectly specifying $q_0$ (column components) increases noise in the inactive indicators' estimates in the same columns as the active indicators, whereas incorrectly specifying $p_0$ (row components) increases noise in the inactive indicators' estimates in the same rows as the active indicators. This again demonstrates that the MPCA model extracts the row and column features separately. When increasing the sample size, this noise reduces, which suggests that the overspecified specified models still converge to the truth. Even with small sample size, the incorrectly specified models can still identify active indicators, with increased noise.

In summary, the misspecified models, even with both $p_0$ and $q_0$ incorrectly specified, can still clearly identify most active indicators of mediation, at the cost of increased noise compared to the correctly specified model. We conjecture that these overspecified models will still be consistent, but with reduced estimation efficiency in small samples.

# Web Appendix I Additional Information on Real Data Application

## I.1 Choosing $p_0$ and $q_0$

To choose the dimension $p_0$ and $q_0$ of the dimension reduction, we consider three approaches: (1) varying $p_0$ and $q_0$ as a sensitivity analysis, and visually checking the impact on the heatmaps of posterior probabilities, (2) choosing a threshold for the percentage of variance explained by the latent features (denoted by VE), similar to PCA, and (3) using the deviance information criteria (DIC). VE can be calculated by the posterior mean of $\sum_{i=1}^n ||\boldsymbol{A}^\top(\boldsymbol{X}_i - \boldsymbol{\mu})\boldsymbol{B}||_F^2 / \sum_{i=1}^n ||\boldsymbol{X}_i - \overline{\boldsymbol{X}}||_F^2$ (Hung et al., 2012), where $||\cdot||_F^2$ is the Frobenius norm. The explained variance proportion should be sufficiently high for the model to be able to capture variation relevant to mediation.

We adopt the conditional approach considered by Celeux et al. (2006) to calculate DIC for Bayesian models with latent variables (definition $\text{DIC}_7$). This definition calculates DIC using the log likelihood of the observed data conditional on the latent variables, averaging over the posterior distribution of both the latent variables and model parameters. In our notation, this is

$$\text{DIC} = -4E_{\boldsymbol{T},\Theta|\mathcal{D}}\left[\sum_{i=1}^n \log f(\boldsymbol{X}_i, Y_i \mid \boldsymbol{T}_i, E_i, \boldsymbol{Z}_i, \Theta)\right] + 2\sum_{i=1}^n \log f(\boldsymbol{X}_i, Y_i \mid \widehat{\boldsymbol{T}}_i, E_i, \boldsymbol{Z}_i, \widehat{\Theta}),$$

where

$$
\begin{aligned}
f(\boldsymbol{X}_i, Y_i \mid \boldsymbol{T}_i, E_i, \boldsymbol{Z}_i, \Theta) &= f(Y_i \mid \boldsymbol{T}_i, E_i, \boldsymbol{Z}_i, \Theta) f(\boldsymbol{X}_i \mid \boldsymbol{T}_i, \Theta) \\
&= p_i^{\mathcal{I}(Y_i=1)}(1-p_i)^{\mathcal{I}(Y_i=0)} \left(\frac{\phi}{2\pi}\right)^{pq/2} \exp\left(-\frac{\phi}{2}\left\|\boldsymbol{X}_i - \boldsymbol{\mu} - \boldsymbol{A}\boldsymbol{T}_i\boldsymbol{B}^\top\right\|_F^2\right) \qquad \text{(I.1)}
\end{aligned}
$$

is the conditional likelihood contribution of one individual given by the full likelihood equation (A.1). $\log f(\boldsymbol{X}_i, Y_i \mid \widehat{\boldsymbol{T}}_i, E_i, \boldsymbol{Z}_i, \widehat{\Theta})$ is the conditional likelihood evaluated at the point estimates $\widehat{\boldsymbol{T}}_i$ and $\widehat{\Theta}$, and it can be calculated by substituting the posterior means of these quantities into Equation (I.1). We note that since some of these quantities are only identifiable up to orthogonal rotations, we instead substitute the posterior means of their corresponding identifiable bi-products or tri-products instead into Equation (I.1). For example, $\boldsymbol{A}$, $\boldsymbol{B}$, and $\boldsymbol{T}_i$ are only identifiable up to orthogonal rotations, so we instead substitute the posterior means of the identifiable tri-product $\boldsymbol{A}\boldsymbol{T}_i\boldsymbol{B}^\top$ into Equation (I.1)

## I.2 Additional Figures

Web Figures I.1 and I.2 show the heatmaps of posterior probabilities for DVH data with threshold $\kappa = 50\%$ and $\kappa = 25\%$ percentiles of the range of the posterior mean mediation quantities for each $p_0$ and $q_0$ specification, respectively. They provide additional evaluations and evidence of the identification performance of the joint model in the application study.

Web Figure I.3 provides a visual evaluation of the convergence of the Gibbs sampling algorithm for the $(p_0, q_0) = (4, 4)$, $(p_0, q_0) = (5, 5)$, and $(p_0, q_0) = (6, 6)$ models in the real data application. Posterior samples generally show clean convergence in the traceplots.

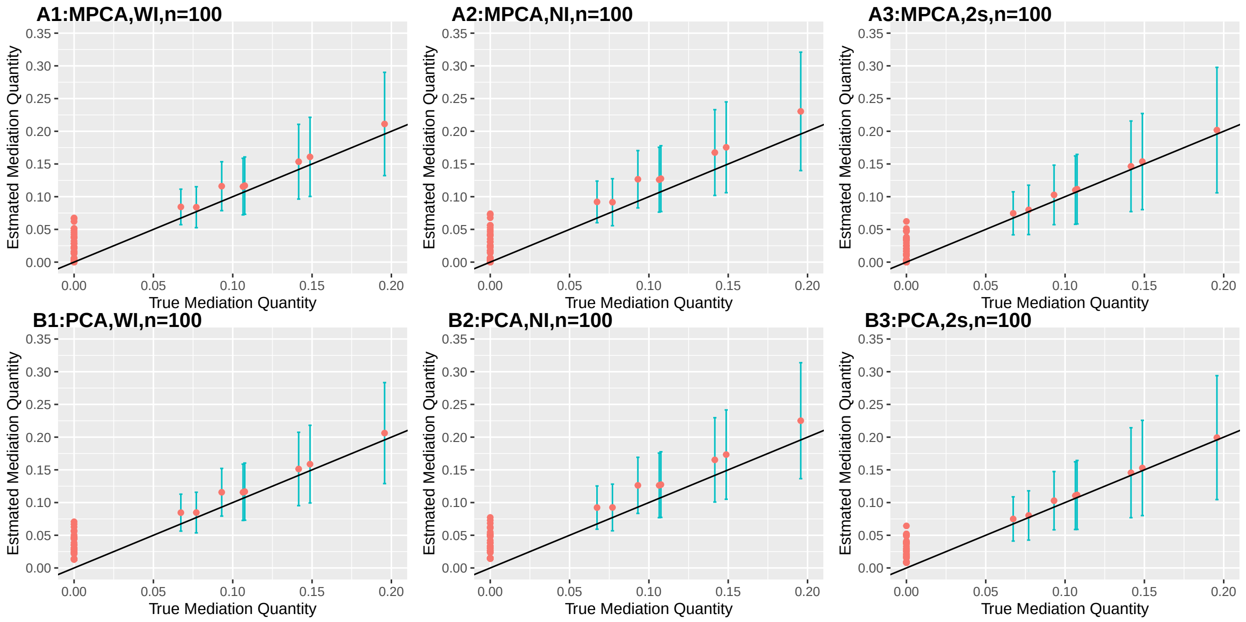


(a) $n = 100$. A1-A3: MPCA models, joint modeling with weakly informative priors, non-informative priors, and two-step method, respectively; B1-B3: PCA models, joint modeling with weakly informative prior, non-informative prior, and two-step method, respectively.

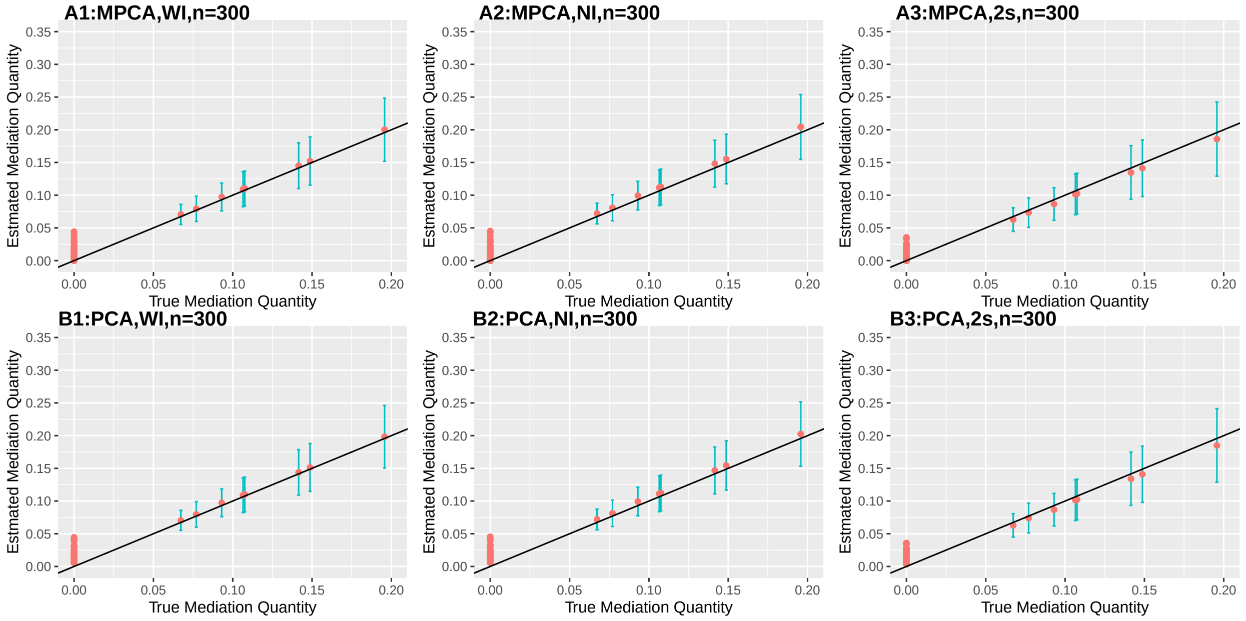


(b) $n = 300$. A1-A3: MPCA models, joint modeling with weakly informative priors, non-informative priors, and two-step method, respectively; B1-B3: PCA models, joint modeling with weakly informative prior, non-informative prior, and two-step method, respectively.

Web Figure G.1: Scatter plots of the mean estimated mediation quantities (red dots) with the black diagonal line and blue error bars (estimates $\pm$ 1-standard deviation across 500 simulation replicates) for different models. WI = weakly informative priors; NI = non-informative priors; 2s = two-step method.

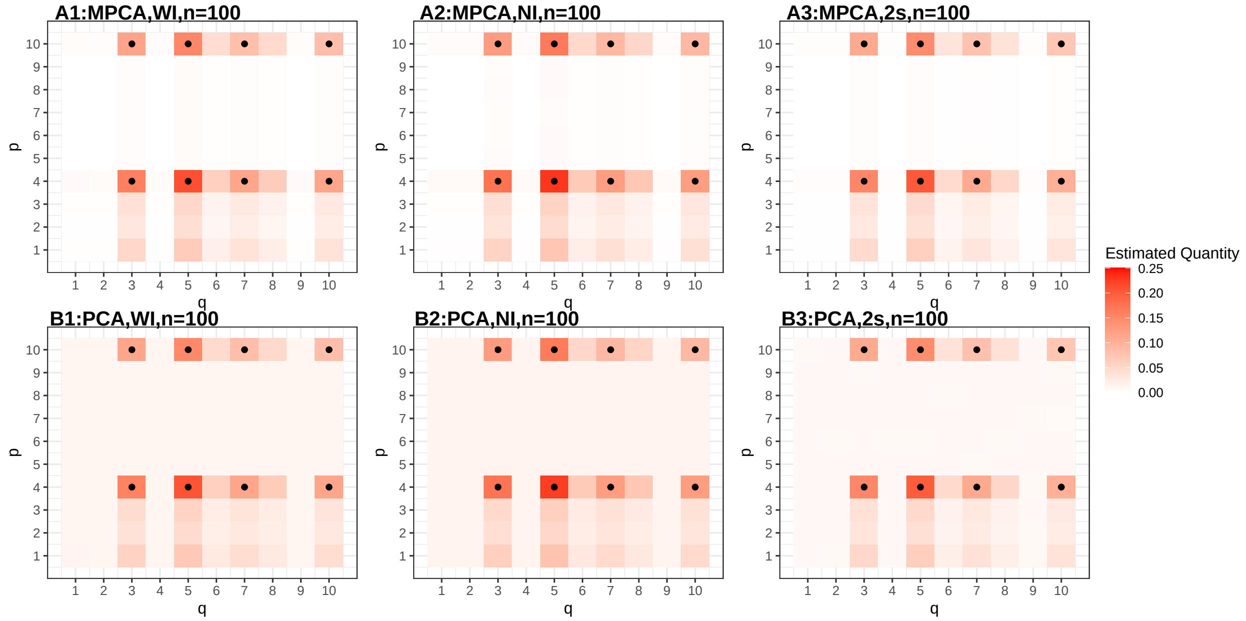


(a) $n = 100$. A1-A3: MPCA models, joint modeling with weakly informative priors, non-informative priors, and two-step method, respectively; B1-B3: PCA models, joint modeling with weakly informative prior, non-informative prior, and two-step method, respectively.

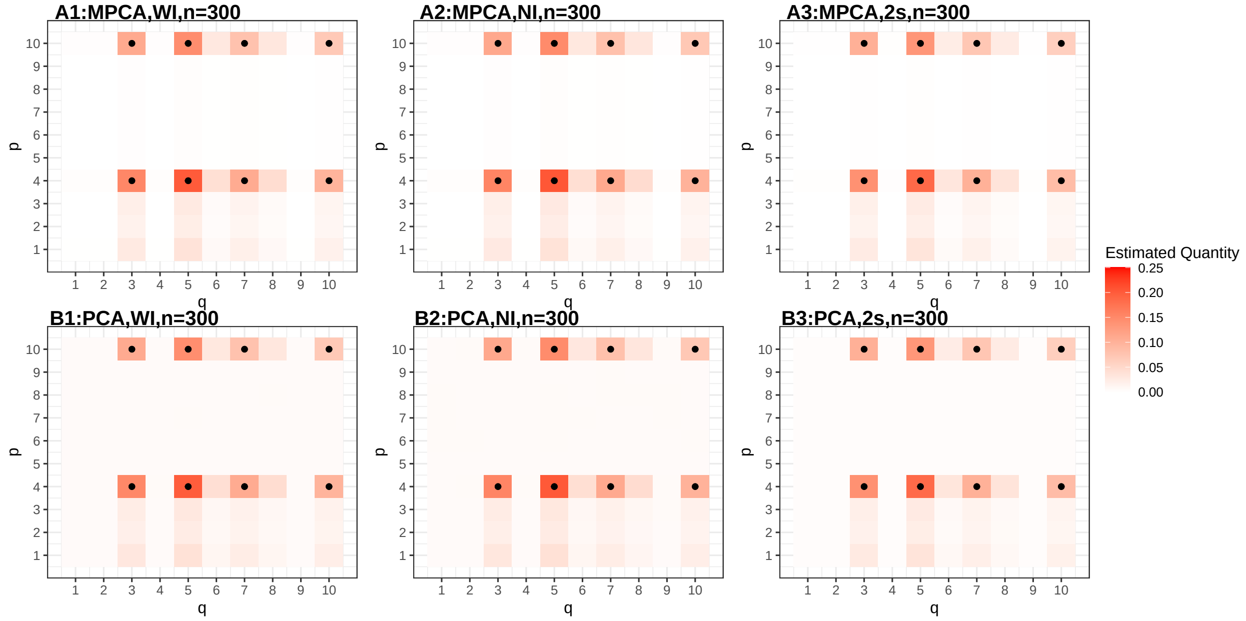


(b) $n = 300$. A1-A3: MPCA models, joint modeling with weakly informative priors, non-informative priors, and two-step method, respectively; B1-B3: PCA models, joint modeling with weakly informative prior, non-informative prior, and two-step method, respectively.

Web Figure G.2: Heatmaps of the estimated mediation quantities with black dots indicating simulated active indicators of mediation. WI = weakly informative priors; NI = non-informative priors; 2s = two-step method.

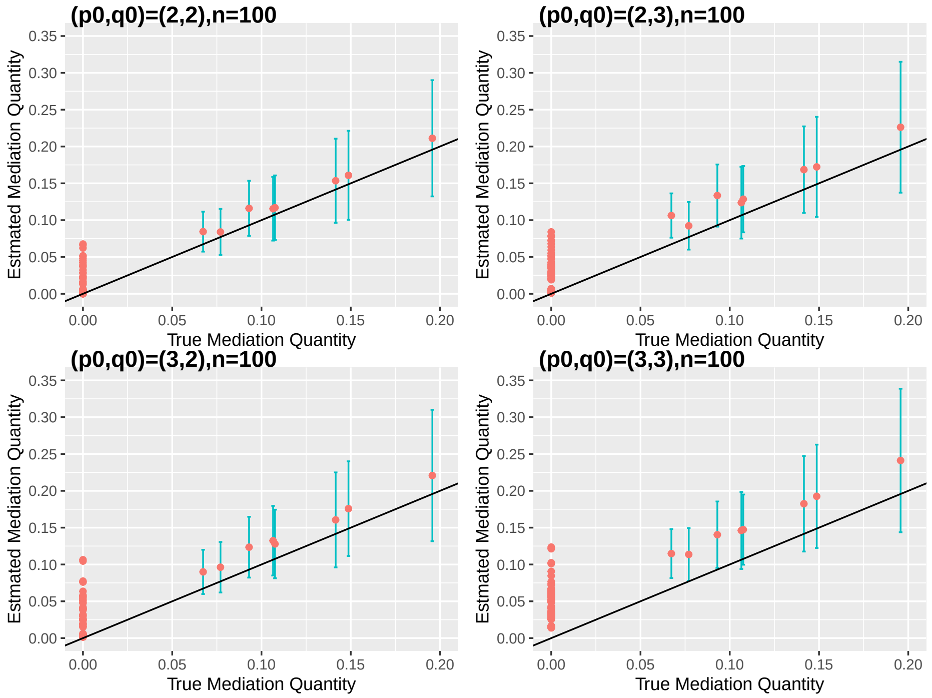


(a) $n = 100$. Top-left Panel: $(p_0, q_0)$ is correctly specified as $(2, 2)$; Top-right, bottom-left, bottom-right Panels: $(p_0, q_0)$ is incorrectly specified as $(2, 3), (3, 2)$ and $(3, 3)$, respectively.

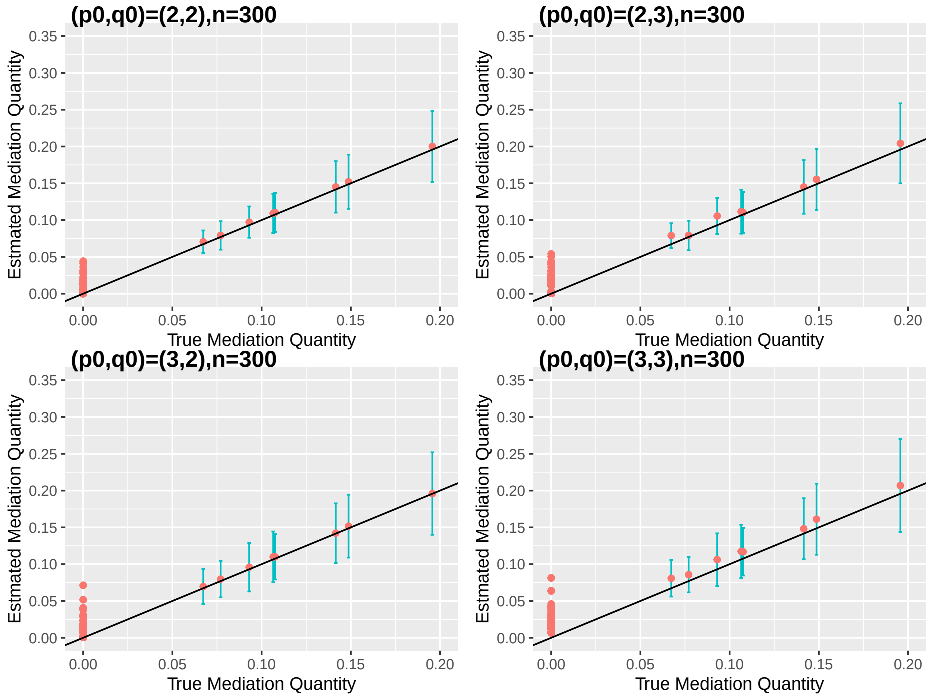


(b) $n = 300$. Top-left Panel: $(p_0, q_0)$ is correctly specified as $(2, 2)$; Top-right, bottom-left, bottom-right Panels: $(p_0, q_0)$ is incorrectly specified as $(2, 3), (3, 2)$ and $(3, 3)$, respectively.

Web Figure H.1: Scatter plots of the mean estimated mediation quantities (red dots) with the black diagonal line and blue error bars (estimates $\pm$ 1-standard deviation across 500 simulation replicates) for different $(p_0, q_0)$ specification.

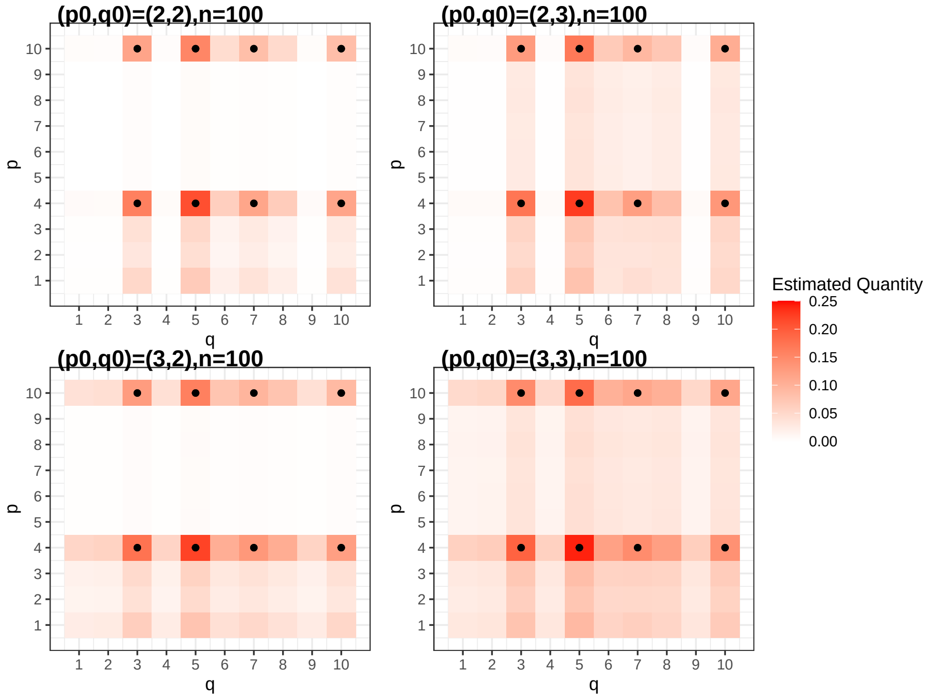


(a) $n = 100$. Top-left Panel: $(p_0, q_0)$ is correctly specified as $(2, 2)$; Top-right, bottom-left, bottom-right Panels: $(p_0, q_0)$ is incorrectly specified as $(2, 3), (3, 2)$ and $(3, 3)$, respectively.

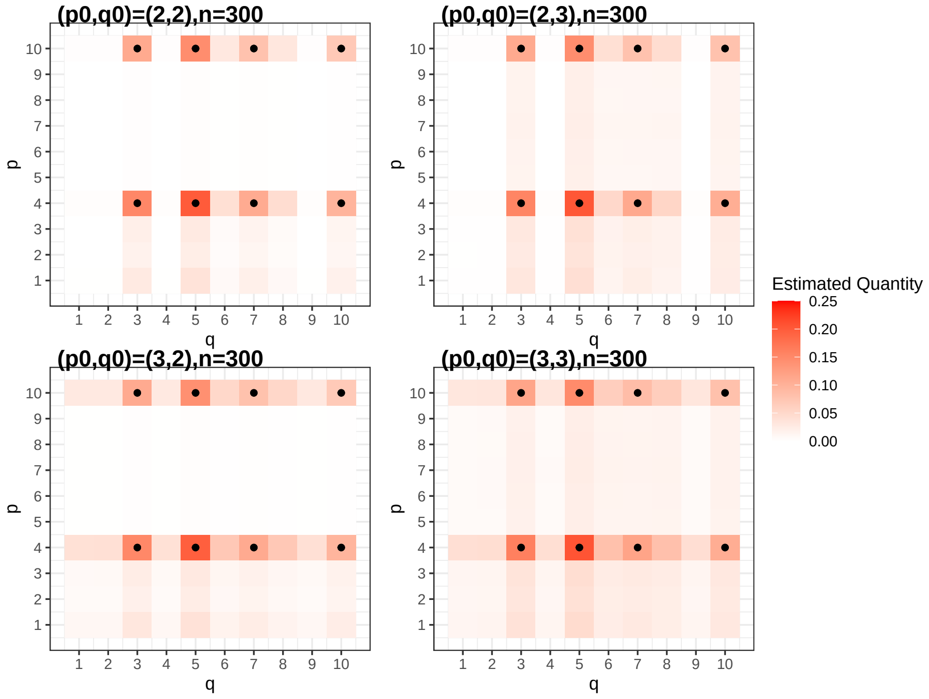


(b) $n = 300$. Top-left Panel: $(p_0, q_0)$ is correctly specified as $(2, 2)$; Top-right, bottom-left, bottom-right Panels: $(p_0, q_0)$ is incorrectly specified as $(2, 3), (3, 2)$ and $(3, 3)$, respectively.

Web Figure H.2: Heatmaps of the estimated mediation quantities with black dots indicating simulated active indicators of mediation for different $(p_0, q_0)$ specification.

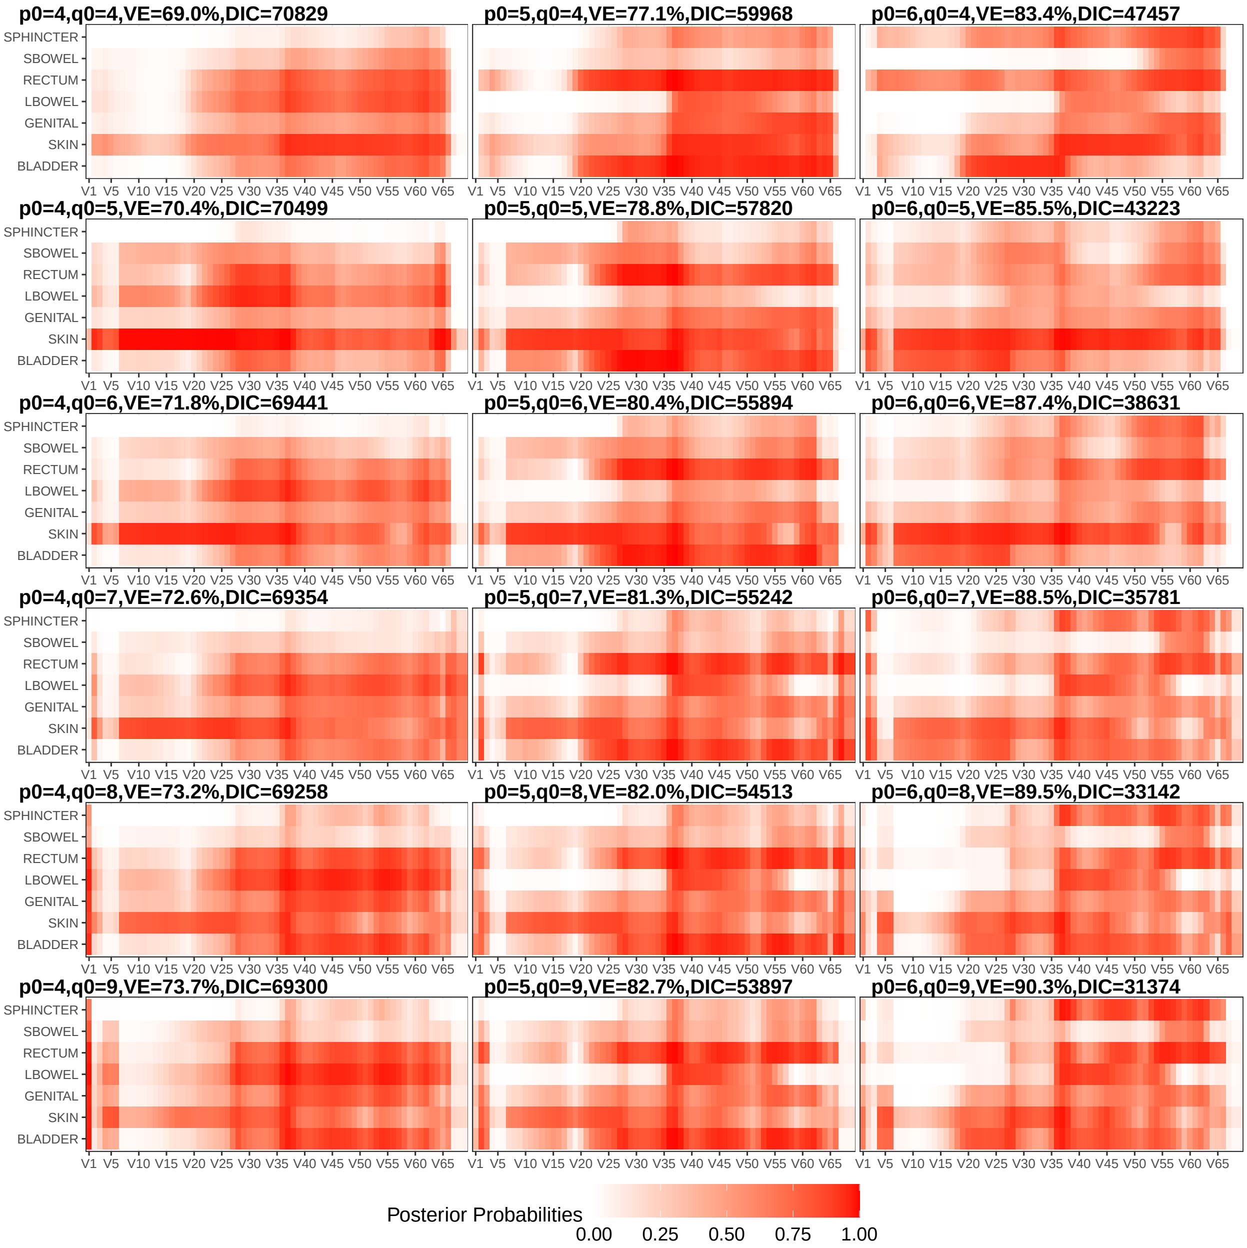


Web Figure I.1: Heatmaps of posterior probabilities for several $p_0$ and $q_0$ specifications in the DVH application. Threshold $\kappa = 50\%$ percentile of the range of the posterior mean mediation quantities for each model. VE = variance explained by latent features, SBOWEL = small bowel, LBOWEL = large bowel.

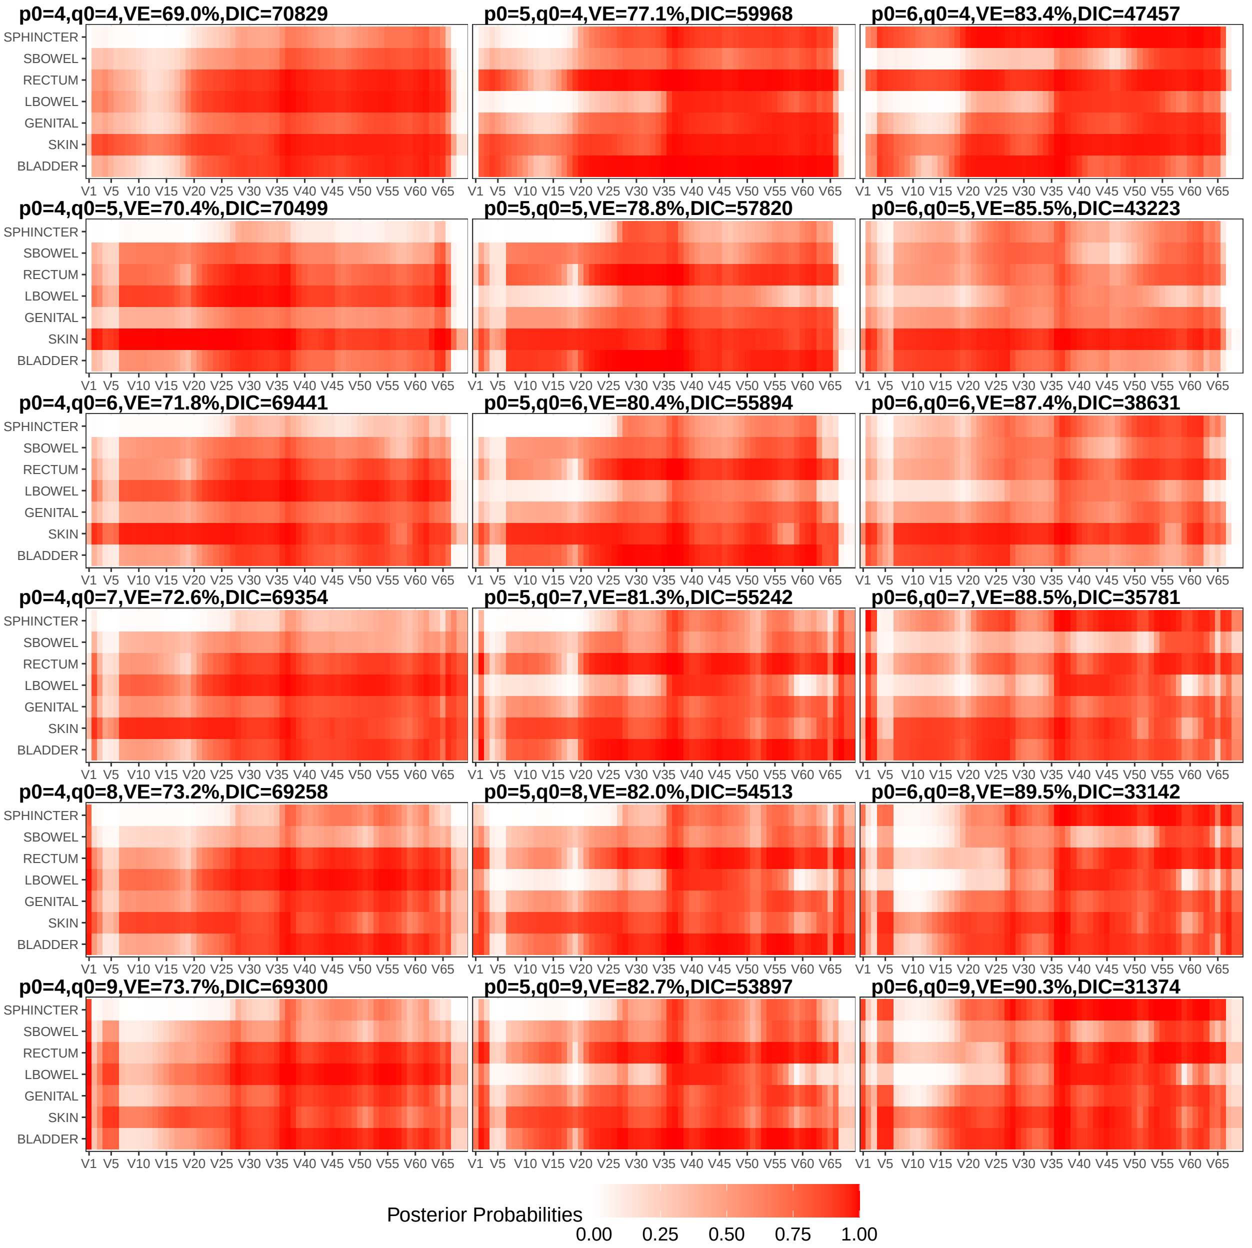


Web Figure I.2: Heatmaps of posterior probabilities for several $p_0$ and $q_0$ specifications in the DVH application. Threshold $\kappa = 25\%$ percentile of the range of the posterior mean mediation quantities for each model. VE = variance explained by latent features, SBOWEL = small bowel, LBOWEL = large bowel.

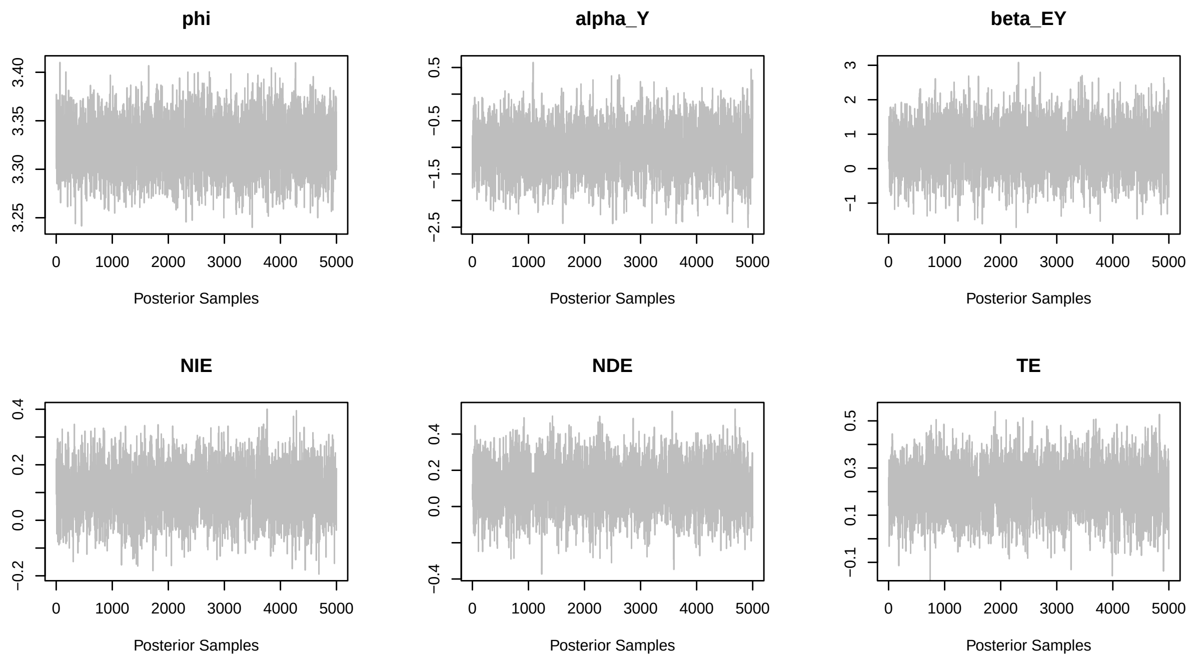


(a) $(p_0, q_0) = (4, 4)$

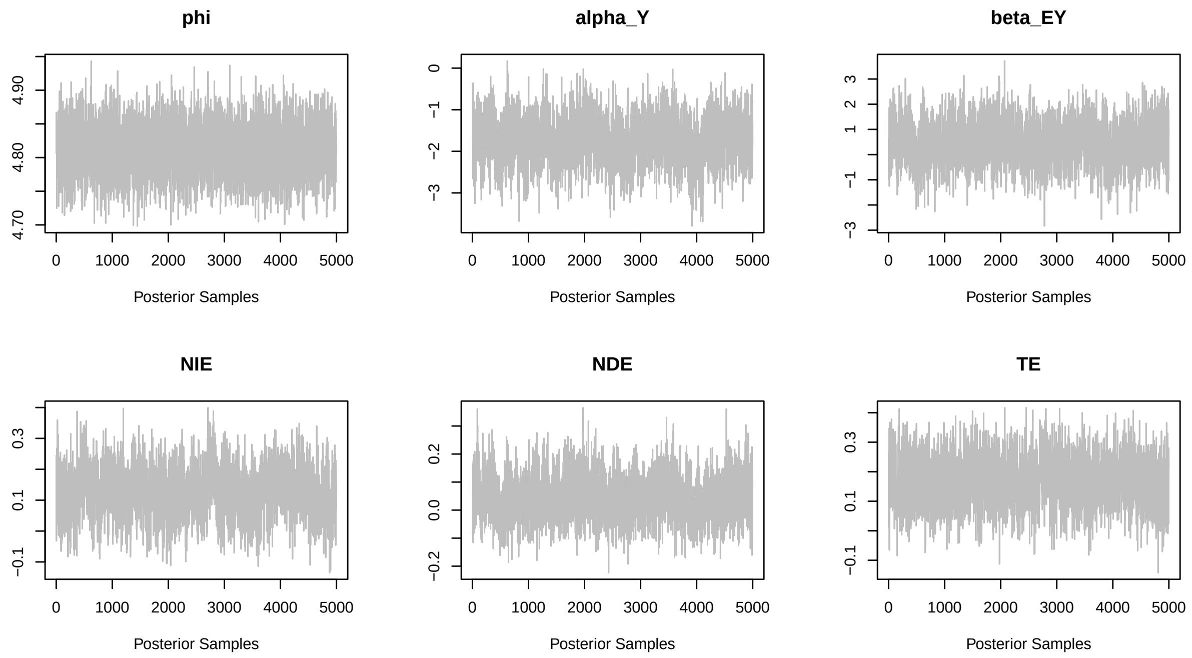


(b) $(p_0, q_0) = (5, 5)$

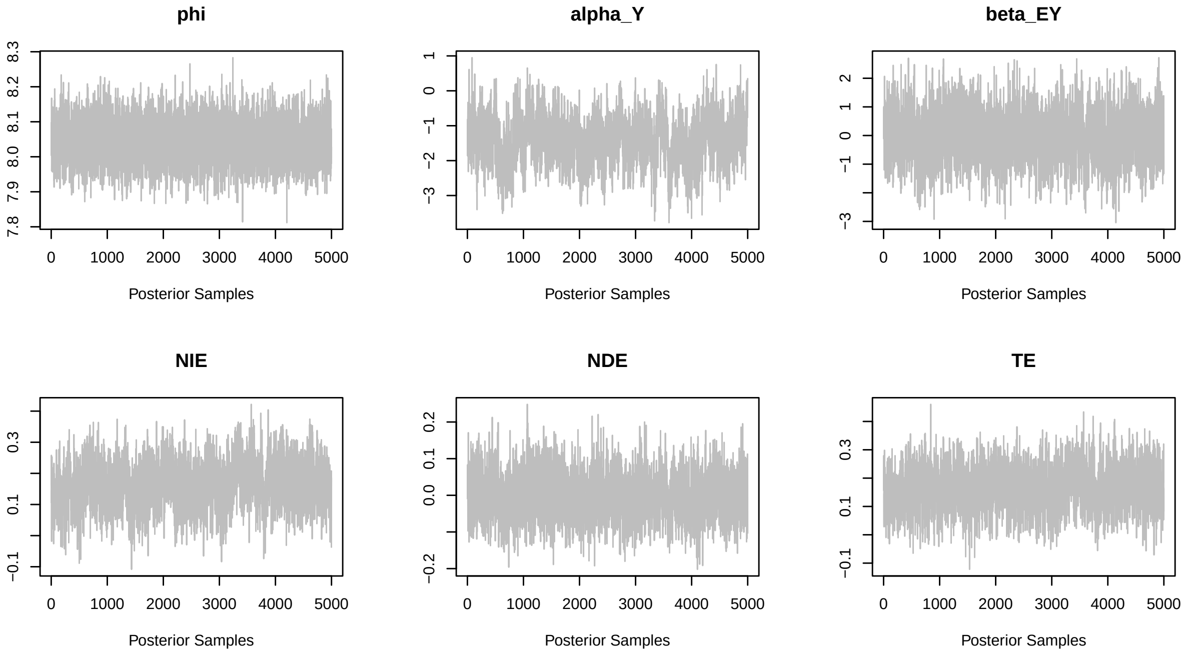


(c) $(p_0, q_0) = (6, 6)$

Web Figure I.3: Traceplots of identifiable parameters and causal decomposition effects in the application study.

# References

Anderson, T. and Rubin, H. (1956). Statistical inference in. In *Proceedings of the Berkeley Symposium on Mathematical Statistics and Probability*, page 111. University of California Press.

Celeux, G., Forbes, F., Robert, C. P., and Titterington, D. M. (2006). Deviance information criteria for missing data models. *Bayesian Analysis*, 1(4):651 – 673.

Derkach, A., Pfeiffer, R. M., Chen, T.-H., and Sampson, J. N. (2019). High dimensional mediation analysis with latent variables. *Biometrics*, 75(3):745–756.

Ding, S. and Cook, R. D. (2014). Dimension folding PCA and PFC for matrix-valued predictors. *Statistica Sinica*, 24(1):463–492.

Hoff, P. D. (2007). Model averaging and dimension selection for the singular value decomposition. *Journal of the American Statistical Association*, 102(478):674–685.

Hung, H., Wu, P., Tu, I., and Huang, S. (2012). On multilinear principal component analysis of order-two tensors. *Biometrika*, 99(3):569–583.

Jiang, B., Petkova, E., Tarpey, T., and Ogden, R. T. (2020). A Bayesian approach to joint modeling of matrix-valued imaging data and treatment outcome with applications to depression studies. *Biometrics*, 76(1):87–97.

Lange, T., Rasmussen, M., and Thygesen, L. C. (2014). Assessing natural direct and indirect effects through multiple pathways. *American journal of epidemiology*, 179(4):513–518.

Li, B., Kim, M. K., and Altman, N. (2010). On dimension folding of matrix- or array-valued statistical objects. *The Annals of Statistics*, 38(2):1094 – 1121.

Lu, H., Plataniotis, K. N., and Venetsanopoulos, A. N. (2008). MPCA: Multilinear principal component analysis of tensor objects. *IEEE transactions on Neural Networks*, 19(1):18–39.

Tipping, M. E. and Bishop, C. M. (1999). Probabilistic principal component analysis. *Journal of the Royal Statistical Society: Series B (Statistical Methodology)*, 61(3):611–622.
