# Supplementary material for: A Bayesian joint model for mediation analysis with matrix-valued mediators
Source: arXiv:2310.00803 source file (2024-09-24)

**$(p_0, q_0) = (2, 2), n = 100$**

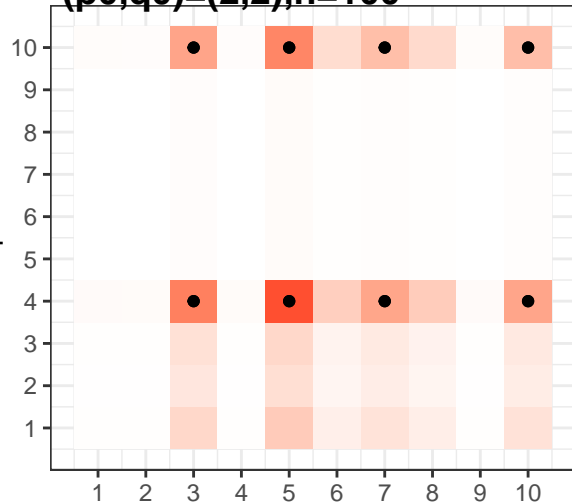

**$(p_0, q_0) = (2, 3), n = 100$**

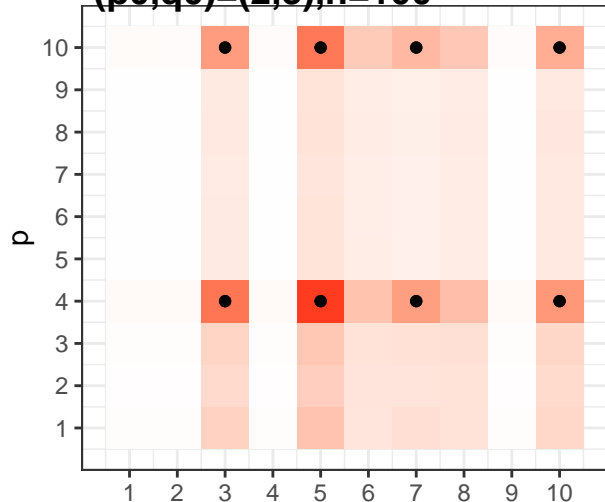

**$(p_0, q_0) = (3, 2), n = 100$**

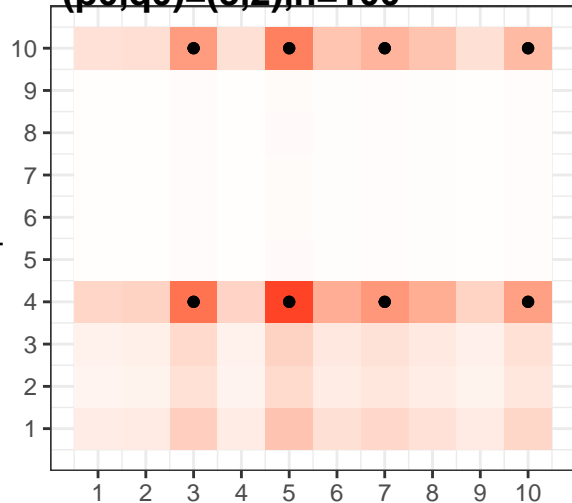

**$(p_0, q_0) = (3, 3), n = 100$**

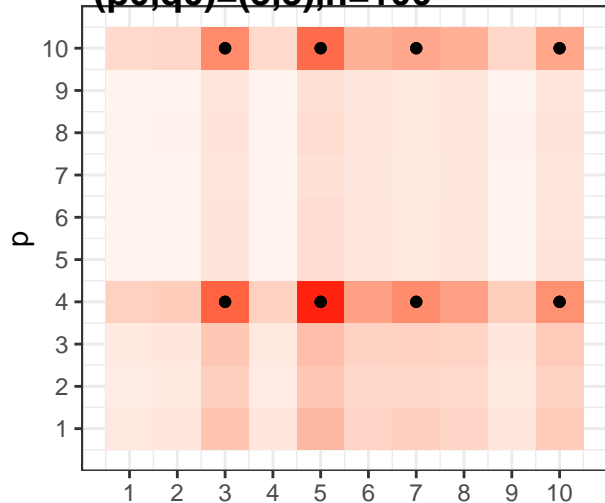

Estimated Quantity

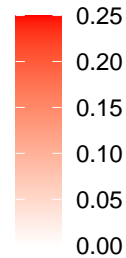

**$(p_0, q_0) = (2, 2), n = 300$**

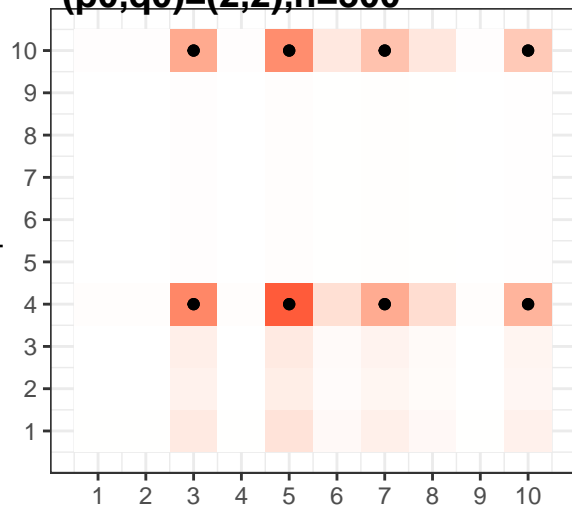

**$(p_0, q_0) = (2, 3), n = 300$**

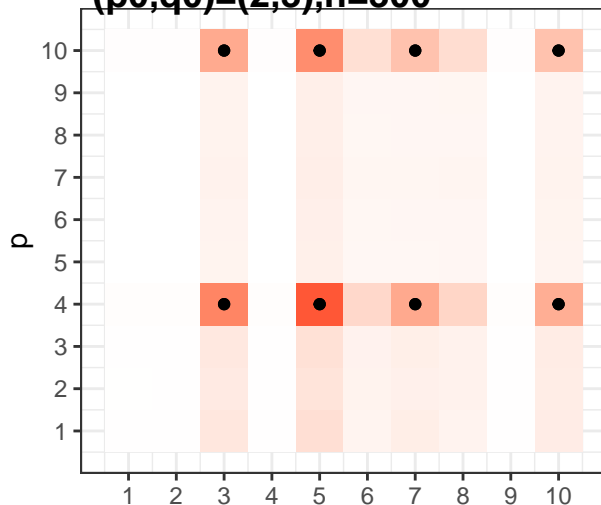

**$(p_0, q_0) = (3, 2), n = 300$**

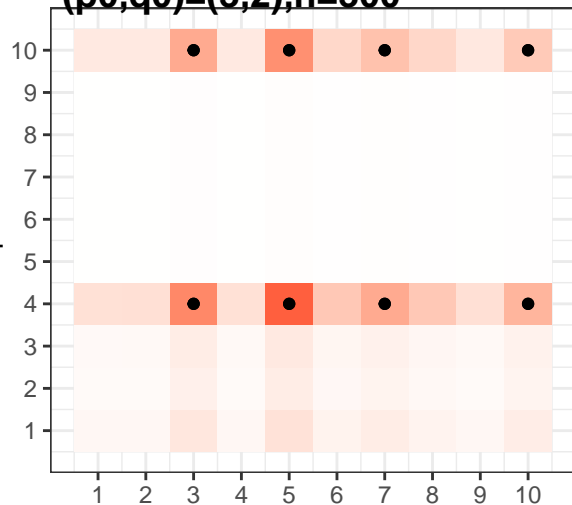

**$(p_0, q_0) = (3, 3), n = 300$**

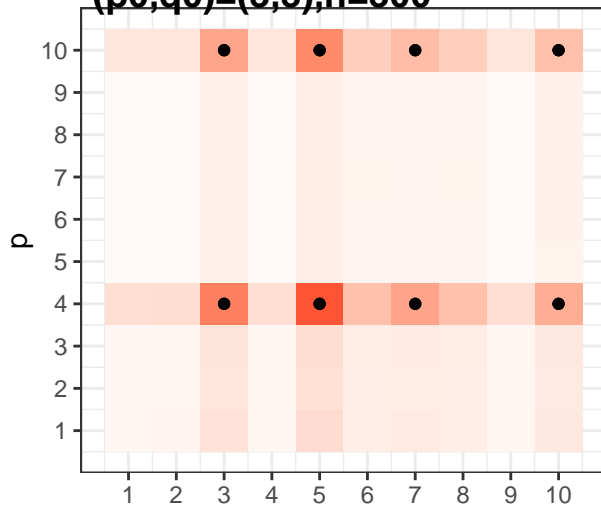

Estimated Quantity

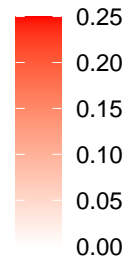

Supplement: Supplementary file 3 [file fig_medQ_mis_appendix.pdf]
