# Supplementary material for: A Bayesian joint model for mediation analysis with matrix-valued mediators
Source: arXiv:2310.00803 source file (2024-09-24)

**A1:MPCA,WI,n=100**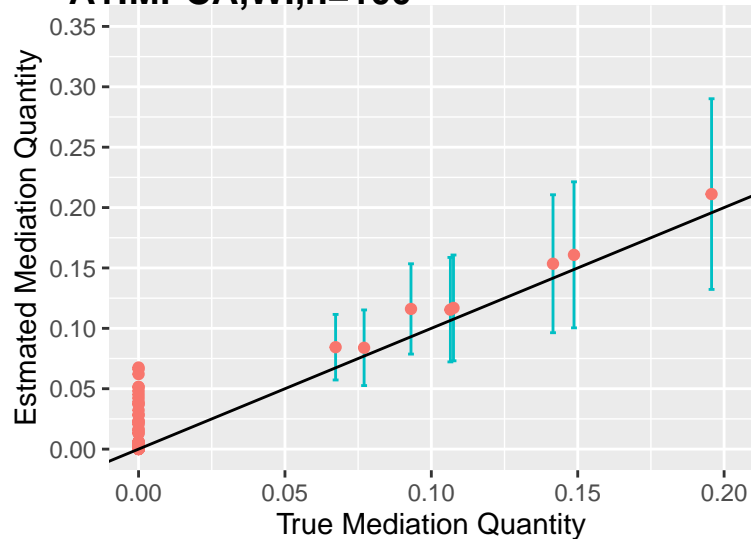**A2:MPCA,NI,n=100**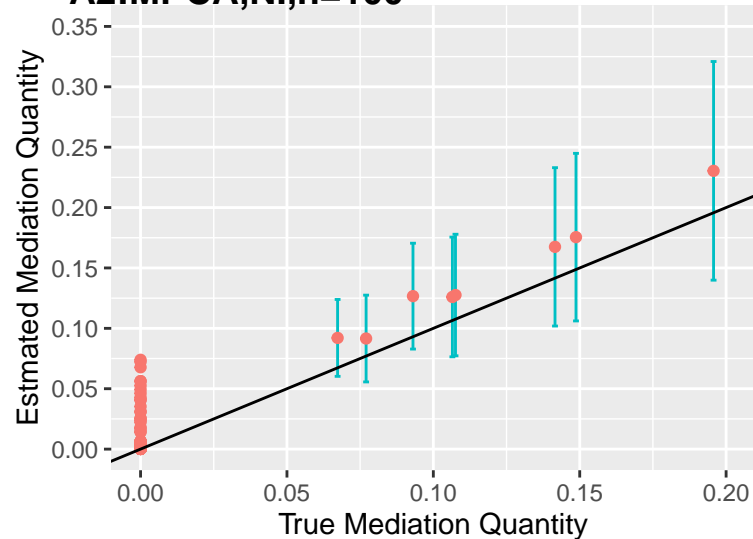**A3:MPCA,2s,n=100**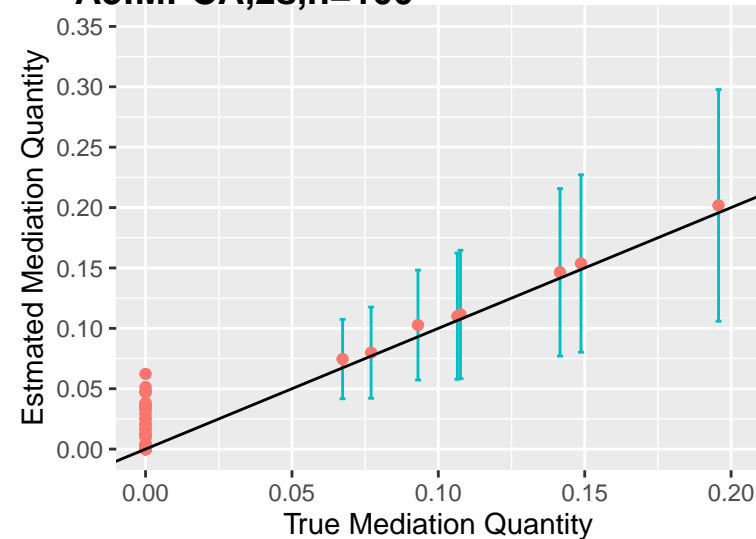**B1:PCA,WI,n=100**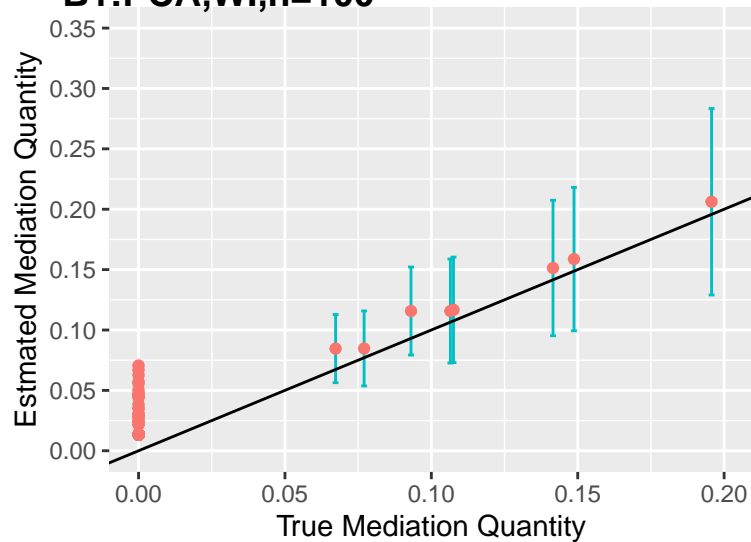**B2:PCA,NI,n=100**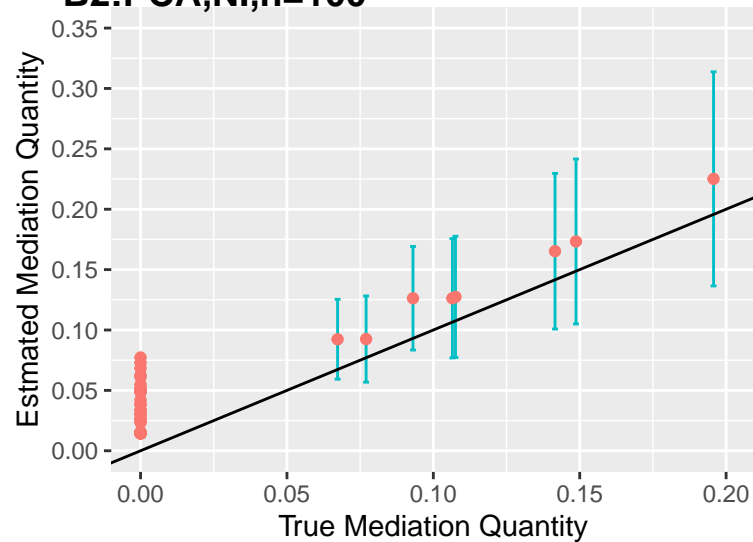**B3:PCA,2s,n=100**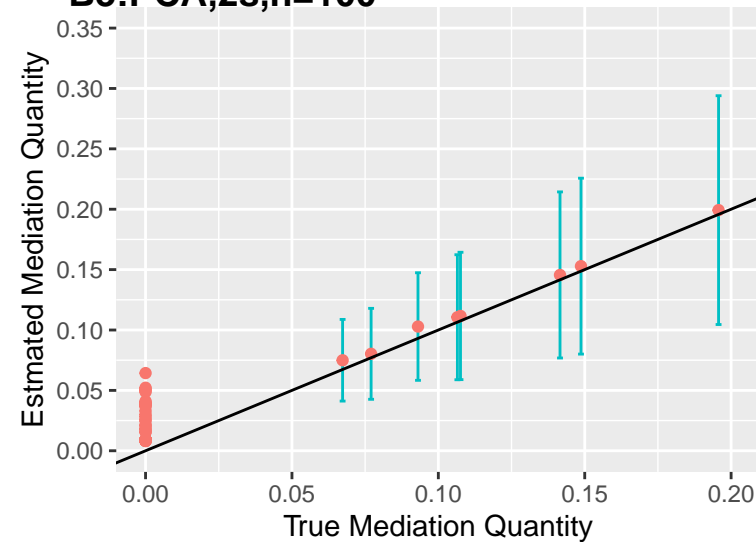

**A1:MPCA,WI,n=300**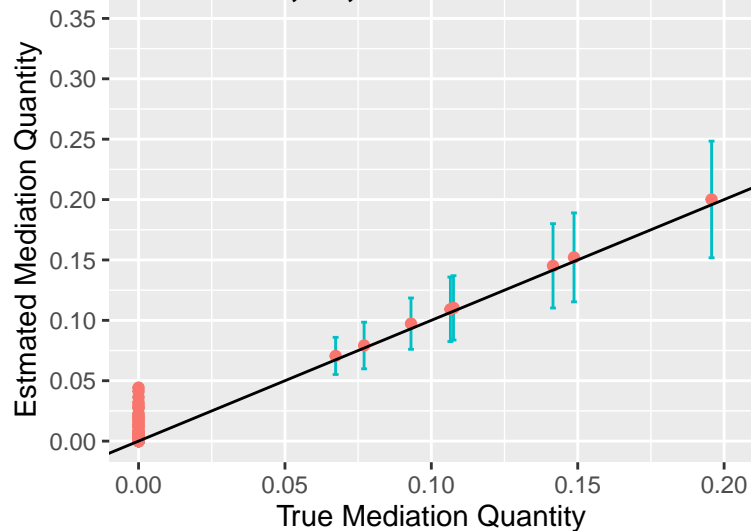**A2:MPCA,NI,n=300**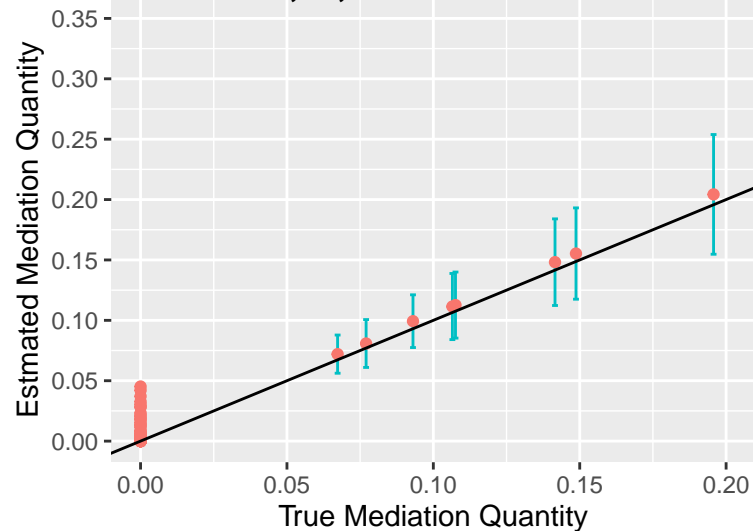**A3:MPCA,2s,n=300**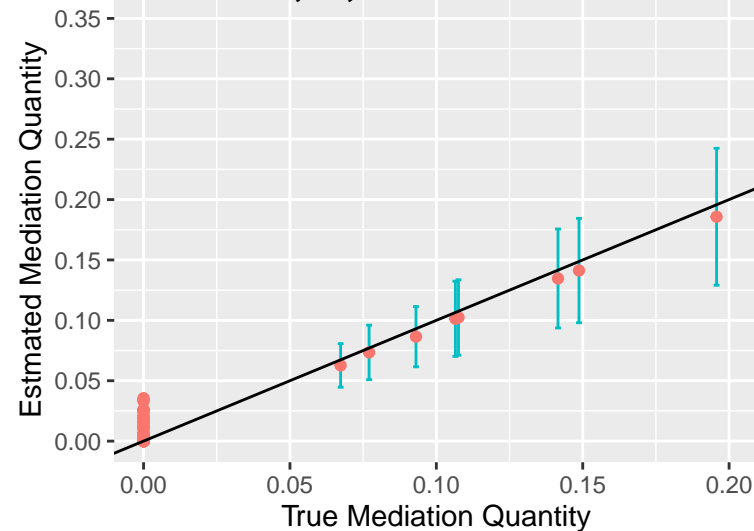**B1:PCA,WI,n=300**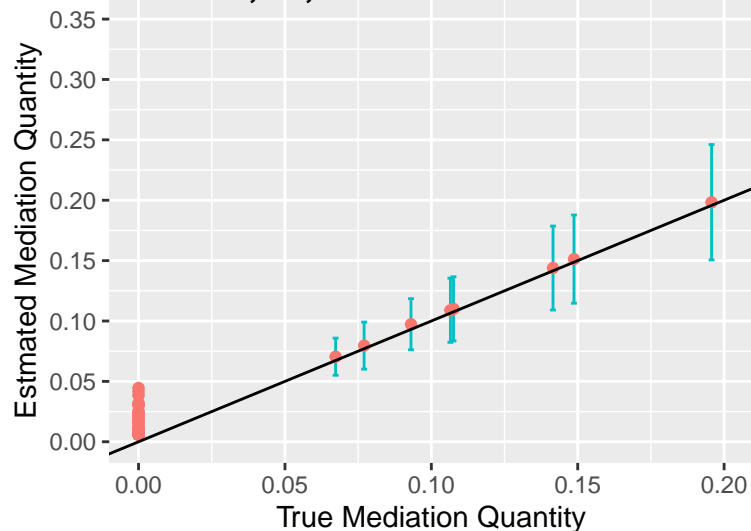**B2:PCA,NI,n=300**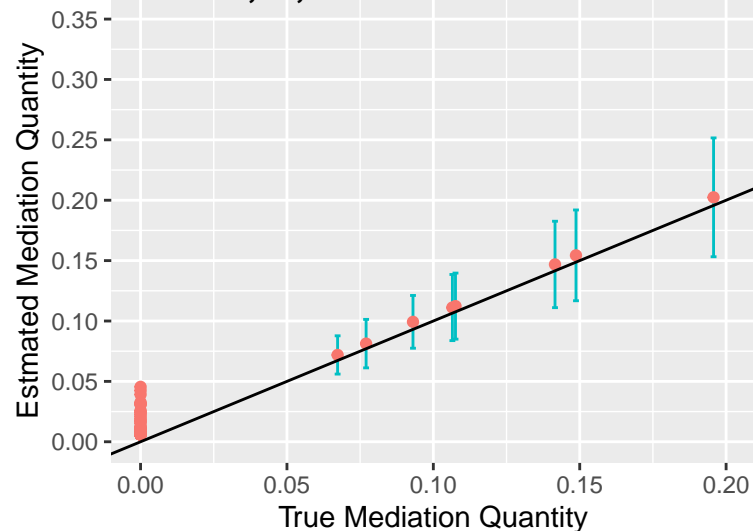**B3:PCA,2s,n=300**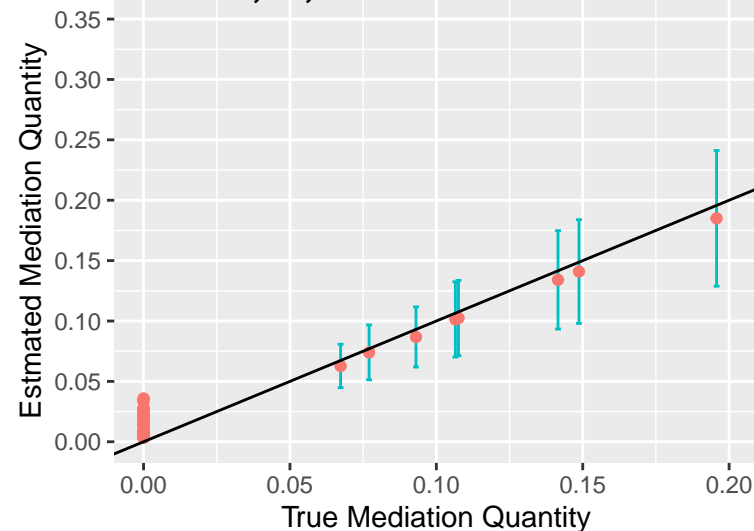

Supplement: Supplementary file 5 [file fig_scatter_pca_mpca_2s_appendix.pdf]
